# Supplementary material for: DyNCA: Real-time Dynamic Texture Synthesis Using Neural Cellular Automata
Source: arXiv:2211.11417 source file (2023-03-30)
Supplement: Supplementary file 1 [file CPEAbl.tex]

\section{Ablation Study for Positional Encoding}
We demonstrate qualitatively and quantitatively that our proposed positional encoding improves the performance of DyNCA.

\subsection{Motion from Vector Field}
In the main paper, we quantitatively show that using Replicate Padding + Cartesian Positional Encoding (CPE) achieves better results compared to other padding strategies without positional encoding. The results provided in the paper were averaged over 10 different target appearances and 4 different structured motion vector fields (Circular, Converge, Diverge, and Hyperbolic). We provide both qualitative and quantitative results for other motion vector fields. We compare DyNCA with CPE to 3 different baselines that use different padding strategies (Zero-Padding, Replicate-Padding, and Circular-Padding) but do not utilize positional encoding. We use the DyNCA-S configuration and train the models with a seed size of $128 \times 128$. 

\subsubsection{Qualitative Analysis}
Figure~\ref{tab:vec-motion-res-more1} shows the qualitative results of our ablation study for positional encoding. The first two rows in Figure~\ref{tab:vec-motion-res-more1} illustrate the 12 different target vector fields we used in our training. We define a \textbf{Structured Vector Field} as a vector field in which either the direction or the magnitude of the motion is position-dependent.
For example, in the \textit{Right acc. Right} and \textit{Right acc. Down} vector fields, the magnitude of the motion depends on the position. In the \textit{Converge}, \textit{Diverge}, \textit{2Block\_X}, \textit{2Block\_Y}, \textit{3Block}, and \textit{4Block} vector fields, the direction of the motion is position-dependent.
And finally, in the \textit{Circular}, and \textit{Hyperbolic} vector fields, both the motion magnitude and motion direction depend on the position.

Figure~\ref{tab:vec-motion-res-more1} shows snapshots of the optic flow for the videos synthesized by the baselines and the final DyNCA configuration utilizing CPE. We can observe that for simple vector fields, such as \textit{Right} and \textit{Up}, all of the baselines fit the motion and generate acceptable results. However, when the target vector field becomes more structured and complex, the baselines fail to learn the correct motion. For example, all the baselines fail when the motion magnitude is position-dependent. Although the DyNCA baselines with zero-padding and replicate padding are able to fit some structured target vector fields such as \textit{Diverge} and \textit{2Block\_X}, we can observe that after resizing the input seed to $256 \times 256$ the baseline fails to generate the correct motion.

\newcommand{\imgmotvec}[1]{\includegraphics[height=100pt]{figures/Experiments/MotionVec/#1}}
\newcolumntype{L}{>{\centering\arraybackslash} m{40pt} } 
\begin{table*}[]
\resizebox{\linewidth}{!}{
\begin{tabular}{Lc||cccccccccccc}
% \toprule
& & \textbf{\Large Right} & 
\textbf{\Large Up} & 
\textbf{{\Large Right acc. Right}} & 
\textbf{{\Large Right acc. Down}} & 
\textbf{\Large Circular }& 
\textbf{\Large Converge} & 
\textbf{\Large Diverge} & 
\textbf{\Large Hyperbolic} & 
\textbf{\Large 2Block\_X} & 
\textbf{\Large 2Block\_Y} & 
\textbf{\Large 3Block} & 
\textbf{\Large 4Block} \\

\multirow{2}{*}[30pt]{\rotatebox{90}{\parbox{3.8cm}{\hspace{30pt} \textbf{{\Huge Target}}}}} &   & 
\imgmotvec{target_symbolic/0.png} & 
\imgmotvec{target_symbolic/270.png} & 
\imgmotvec{target_symbolic/grad_0_0.png} & 
\imgmotvec{target_symbolic/grad_0_90.png} & 
\imgmotvec{target_symbolic/circular.png} & 
\imgmotvec{target_symbolic/concentrate.png} & 
\imgmotvec{target_symbolic/diverge.png} & 
\imgmotvec{target_symbolic/hyperbolic.png} & 
\imgmotvec{target_symbolic/2block_x.png} & 
\imgmotvec{target_symbolic/2block_y.png} & 
\imgmotvec{target_symbolic/3block.png} & 
\imgmotvec{target_symbolic/4block.png} \\
 & & 
\imgmotvec{target_color/0.png} & 
\imgmotvec{target_color/270.png} & 
\imgmotvec{target_color/grad_0_0.png} & 
\imgmotvec{target_color/grad_0_90.png} & 
\imgmotvec{target_color/circular.png} & 
\imgmotvec{target_color/concentrate.png} & 
\imgmotvec{target_color/diverge.png} & 
\imgmotvec{target_color/hyperbolic.png} & 
\imgmotvec{target_color/2block_x.png} & 
\imgmotvec{target_color/2block_y.png} & 
\imgmotvec{target_color/3block.png} & 
\imgmotvec{target_color/4block.png} \\
\midrule
\midrule
\midrule
\multirow{4}{*}[-20pt]{\rotatebox{90}{\parbox{8.0cm}{\hspace{30pt} \textbf{{\Huge Seed Size $128 \times 128$}}}}} &  \rotatebox{90}{\parbox{3.5cm}{\hspace{30pt}\textbf{{\LARGE CPE}  }}} & 
\imgmotvec{synthesized_cpe/chequered_0121/0.png} & 
\imgmotvec{synthesized_cpe/chequered_0121/270.png} & 
\imgmotvec{synthesized_cpe/chequered_0121/grad_0_0.png} & 
\imgmotvec{synthesized_cpe/chequered_0121/grad_0_90.png} & 
\imgmotvec{synthesized_cpe/chequered_0121/circular.png} & 
\imgmotvec{synthesized_cpe/chequered_0121/concentrate.png} & 
\imgmotvec{synthesized_cpe/chequered_0121/diverge.png} & 
\imgmotvec{synthesized_cpe/chequered_0121/hyperbolic.png} & 
\imgmotvec{synthesized_cpe/chequered_0121/2block_x.png} & 
\imgmotvec{synthesized_cpe/chequered_0121/2block_y.png} & 
\imgmotvec{synthesized_cpe/chequered_0121/3block.png} & 
\imgmotvec{synthesized_cpe/chequered_0121/4block.png} \\
 & \rotatebox{90}{\parbox{3.5cm}{\hspace{30pt}\textbf{{\LARGE Zero}  }}} & 
\imgmotvec{synthesized_zero/chequered_0121/0.png} & 
\imgmotvec{synthesized_zero/chequered_0121/270.png} & 
\imgmotvec{synthesized_zero/chequered_0121/grad_0_0.png} & 
\imgmotvec{synthesized_zero/chequered_0121/grad_0_90.png} & 
\imgmotvec{synthesized_zero/chequered_0121/circular.png} & 
\imgmotvec{synthesized_zero/chequered_0121/concentrate.png} & 
\imgmotvec{synthesized_zero/chequered_0121/diverge.png} & 
\imgmotvec{synthesized_zero/chequered_0121/hyperbolic.png} & 
\imgmotvec{synthesized_zero/chequered_0121/2block_x.png} & 
\imgmotvec{synthesized_zero/chequered_0121/2block_y.png} & 
\imgmotvec{synthesized_zero/chequered_0121/3block.png} & 
\imgmotvec{synthesized_zero/chequered_0121/4block.png} \\
 & \rotatebox{90}{\parbox{3.5cm}{\hspace{15pt}\textbf{{\LARGE Replicate}  }}} & 
\imgmotvec{synthesized_replicate/chequered_0121/0.png} & 
\imgmotvec{synthesized_replicate/chequered_0121/270.png} & 
\imgmotvec{synthesized_replicate/chequered_0121/grad_0_0.png} & 
\imgmotvec{synthesized_replicate/chequered_0121/grad_0_90.png} & 
\imgmotvec{synthesized_replicate/chequered_0121/circular.png} & 
\imgmotvec{synthesized_replicate/chequered_0121/concentrate.png} & 
\imgmotvec{synthesized_replicate/chequered_0121/diverge.png} & 
\imgmotvec{synthesized_replicate/chequered_0121/hyperbolic.png} & 
\imgmotvec{synthesized_replicate/chequered_0121/2block_x.png} & 
\imgmotvec{synthesized_replicate/chequered_0121/2block_y.png} & 
\imgmotvec{synthesized_replicate/chequered_0121/3block.png} & 
\imgmotvec{synthesized_replicate/chequered_0121/4block.png} \\
 & \rotatebox{90}{\parbox{3.5cm}{\hspace{20pt}\textbf{{\LARGE Circular}}}} & 
\imgmotvec{synthesized_circular/chequered_0121/0.png} & 
\imgmotvec{synthesized_circular/chequered_0121/270.png} & 
\imgmotvec{synthesized_circular/chequered_0121/grad_0_0.png} & 
\imgmotvec{synthesized_circular/chequered_0121/grad_0_90.png} & 
\imgmotvec{synthesized_circular/chequered_0121/circular.png} & 
\imgmotvec{synthesized_circular/chequered_0121/concentrate.png} & 
\imgmotvec{synthesized_circular/chequered_0121/diverge.png} & 
\imgmotvec{synthesized_circular/chequered_0121/hyperbolic.png} & 
\imgmotvec{synthesized_circular/chequered_0121/2block_x.png} & 
\imgmotvec{synthesized_circular/chequered_0121/2block_y.png} & 
\imgmotvec{synthesized_circular/chequered_0121/3block.png} & 
\imgmotvec{synthesized_circular/chequered_0121/4block.png} \\
\midrule
\midrule
\midrule
\multirow{4}{*}[-20pt]{\rotatebox{90}{\parbox{8.0cm}{\hspace{30pt} \textbf{{\Huge  Seed Size $256 \times 256$}}}}} &  \rotatebox{90}{\parbox{3.5cm}{\hspace{30pt}\textbf{{\LARGE CPE}  }}} & 
\imgmotvec{synthesized_cpe_large/chequered_0121/0.png} & 
\imgmotvec{synthesized_cpe_large/chequered_0121/270.png} & 
\imgmotvec{synthesized_cpe_large/chequered_0121/grad_0_0.png} & 
\imgmotvec{synthesized_cpe_large/chequered_0121/grad_0_90.png} & 
\imgmotvec{synthesized_cpe_large/chequered_0121/circular.png} & 
\imgmotvec{synthesized_cpe_large/chequered_0121/concentrate.png} & 
\imgmotvec{synthesized_cpe_large/chequered_0121/diverge.png} & 
\imgmotvec{synthesized_cpe_large/chequered_0121/hyperbolic.png} & 
\imgmotvec{synthesized_cpe_large/chequered_0121/2block_x.png} & 
\imgmotvec{synthesized_cpe_large/chequered_0121/2block_y.png} & 
\imgmotvec{synthesized_cpe_large/chequered_0121/3block.png} & 
\imgmotvec{synthesized_cpe_large/chequered_0121/4block.png} \\
 & \rotatebox{90}{\parbox{3.5cm}{\hspace{30pt}\textbf{{\LARGE Zero}  }}} & 
\imgmotvec{synthesized_zero_large/chequered_0121/0.png} & 
\imgmotvec{synthesized_zero_large/chequered_0121/270.png} & 
\imgmotvec{synthesized_zero_large/chequered_0121/grad_0_0.png} & 
\imgmotvec{synthesized_zero_large/chequered_0121/grad_0_90.png} & 
\imgmotvec{synthesized_zero_large/chequered_0121/circular.png} & 
\imgmotvec{synthesized_zero_large/chequered_0121/concentrate.png} & 
\imgmotvec{synthesized_zero_large/chequered_0121/diverge.png} & 
\imgmotvec{synthesized_zero_large/chequered_0121/hyperbolic.png} & 
\imgmotvec{synthesized_zero_large/chequered_0121/2block_x.png} & 
\imgmotvec{synthesized_zero_large/chequered_0121/2block_y.png} & 
\imgmotvec{synthesized_zero_large/chequered_0121/3block.png} & 
\imgmotvec{synthesized_zero_large/chequered_0121/4block.png} \\
 & \rotatebox{90}{\parbox{3.5cm}{\hspace{15pt}\textbf{{\LARGE Replicate}  }}} & 
\imgmotvec{synthesized_replicate_large/chequered_0121/0.png} & 
\imgmotvec{synthesized_replicate_large/chequered_0121/270.png} & 
\imgmotvec{synthesized_replicate_large/chequered_0121/grad_0_0.png} & 
\imgmotvec{synthesized_replicate_large/chequered_0121/grad_0_90.png} & 
\imgmotvec{synthesized_replicate_large/chequered_0121/circular.png} & 
\imgmotvec{synthesized_replicate_large/chequered_0121/concentrate.png} & 
\imgmotvec{synthesized_replicate_large/chequered_0121/diverge.png} & 
\imgmotvec{synthesized_replicate_large/chequered_0121/hyperbolic.png} & 
\imgmotvec{synthesized_replicate_large/chequered_0121/2block_x.png} & 
\imgmotvec{synthesized_replicate_large/chequered_0121/2block_y.png} & 
\imgmotvec{synthesized_replicate_large/chequered_0121/3block.png} & 
\imgmotvec{synthesized_replicate_large/chequered_0121/4block.png} \\
 & \rotatebox{90}{\parbox{3.5cm}{\hspace{20pt}\textbf{{\LARGE Circular}  }}} & 
\imgmotvec{synthesized_circular_large/chequered_0121/0.png} & 
\imgmotvec{synthesized_circular_large/chequered_0121/270.png} & 
\imgmotvec{synthesized_circular_large/chequered_0121/grad_0_0.png} & 
\imgmotvec{synthesized_circular_large/chequered_0121/grad_0_90.png} & 
\imgmotvec{synthesized_circular_large/chequered_0121/circular.png} & 
\imgmotvec{synthesized_circular_large/chequered_0121/concentrate.png} & 
\imgmotvec{synthesized_circular_large/chequered_0121/diverge.png} & 
\imgmotvec{synthesized_circular_large/chequered_0121/hyperbolic.png} & 
\imgmotvec{synthesized_circular_large/chequered_0121/2block_x.png} & 
\imgmotvec{synthesized_circular_large/chequered_0121/2block_y.png} & 
\imgmotvec{synthesized_circular_large/chequered_0121/3block.png} & 
\imgmotvec{synthesized_circular_large/chequered_0121/4block.png} \\
\end{tabular}
}
\captionof{figure}{Qualitative comparison of DyNCA baselines with different padding strategies and with the proposed DyNCA model with Cartesian Positional Encoding (CPE). We observe that the DyNCA with CPE  better fits the target motion. Moreover, the model using CPE is able to synthesize the correct motion regardless of the seed size. The target appearance used is chequered\_0121 from the DTD\cite{dtd} dataset.}
\label{tab:vec-motion-res-more1}
\end{table*}

\subsubsection{Quantitative Analysis}
For the quantitative results, we use the same DyNCA-S configuration and train the baselines for all 12 different target fields on the following 10 target appearance textures: \textit{bubbly\_0101}, \textit{chequered\_0121}, \textit{fibrous\_0145}, \textit{cracked\_0085}, \textit{interlaced\_0172}, \textit{water\_3}, \textit{smoke\_2}, \textit{smoke\_plume\_1}, \textit{calm\_water\_4}, and \textit{sea\_2}. To evaluate the motion direction loss $\mathcal{L}_{dir}$ and motion magnitude loss $\mathcal{L}_{norm}$, we synthesize a 330 frame video and exclude the first 30 frames. We then feed the remaining 300 frames into the optic flow prediction network provided in \cite{two_stream} and compare the estimated optic flow with the target vector fields. We average the losses over the 300 frames and over all of the target appearances and report the results in Table~\ref{tab:motion-vec-ablation-quantitative}. The results show that for simpler vector fields such as \textit{Right} and \textit{Up}, circular padding works better than CPE. However, for more complex and structured vector fields, CPE achieves better results both in terms of motion direction loss $\mathcal{L}_{dir}$ and motion magnitude loss $\mathcal{L}_{norm}$. 

% Please add the following required packages to your document preamble:
% \usepackage{multirow}

\begin{table*}[]
\resizebox{\linewidth}{!}{
\begin{tabular}{ccc||cccccccccccc}
\toprule
\textbf{\begin{tabular}[c]{@{}c@{}}Seed \\ Size\end{tabular}}            & \textbf{Loss}         & \textbf{\textbf{Config}} & \textbf{Right}  & \textbf{Up}    & \textbf{\begin{tabular}[c]{@{}c@{}}Right \\ acc. Right\end{tabular}} & \textbf{\begin{tabular}[c]{@{}c@{}}Right \\ acc. Down\end{tabular}} & \textbf{Circular} & \textbf{Converge} & \textbf{Diverge} & \textbf{Hyperbolic} & \textbf{2Block\_X} & \textbf{2Block\_Y} & \textbf{3Block} & \textbf{4Block} \\
\midrule\midrule
\multirow{8}{*}{
\rotatebox{90}{\parbox{3.5cm}{\hspace{30pt} \textbf{$128 \times 128$}}}} & \multirow{4}{*}{$\mathcal{L}_{dir}$}  & CPE                                                              & 0.027          & 0.032          & 0.055                                                                & 0.049                                                               & \textbf{0.048}    & \textbf{0.072}    & \textbf{0.075}   & \textbf{0.053}      & \textbf{0.102}     & \textbf{0.085}     & \textbf{0.107}  & \textbf{0.104}  \\
                              &                       & Zero                                                             & 0.035          & 0.032          & 0.052                                                                & 0.059                                                               & 0.124             & 0.241             & 0.165            & 0.116               & 0.170              & 0.169              & 0.326           & 0.261           \\
                              &                       & Replicate                                                        & 0.024          & 0.033          & 0.054                                                                & 0.047                                                               & 0.241             & 0.339             & 0.344            & 0.345               & 0.289              & 0.365              & 0.336           & 0.452           \\
                              &                       & Circular                                                         & \textbf{0.022} & \textbf{0.027} & \textbf{0.025}                                                       & \textbf{0.025}                                                      & 0.979             & 0.997             & 0.994            & 0.985               & 0.985              & 0.998              & 0.659           & 0.988           \\ \cline{2-15} 
                              & \multirow{4}{*}{$\mathcal{L}_{norm}$} & CPE                                                              & 0.227          & 0.183          & \textbf{0.251}                                                       & \textbf{0.246}                                                      & \textbf{0.233}    & \textbf{0.230}    & \textbf{0.229}   & \textbf{0.249}      & \textbf{0.268}     & \textbf{0.232}     & 0.251           & \textbf{0.229}  \\
                              &                       & Zero                                                             & 0.238          & 0.182          & 0.339                                                                & 0.303                                                               & 0.300             & 0.312             & 0.263            & 0.307               & 0.318              & 0.277              & 0.279           & 0.273           \\
                              &                       & Replicate                                                        & \textbf{0.201} & 0.190          & 0.378                                                                & 0.330                                                               & 0.371             & 0.301             & 0.344            & 0.438               & 0.341              & 0.350              & 0.284           & 0.330           \\
                              &                       & Circular                                                         & 0.213          & \textbf{0.153} & 0.551                                                                & 0.555                                                               & 0.618             & 0.651             & 0.531            & 0.759               & 0.837              & 0.819              & \textbf{0.179}  & 0.651           \\ \midrule
                              \midrule
\multirow{8}{*}{
\rotatebox{90}{\parbox{3.5cm}{\hspace{30pt} \textbf{$256 \times 256$}}}} & \multirow{4}{*}{$\mathcal{L}_{dir}$}  & CPE                                                              & 0.021          & 0.026          & 0.044                                                                & 0.045                                                               & \textbf{0.050}    & \textbf{0.059}    & \textbf{0.058}   & \textbf{0.047}      & \textbf{0.089}     & \textbf{0.068}     & \textbf{0.095}  & \textbf{0.098}  \\
                              &                       & Zero                                                             & 0.023          & 0.024          & 0.037                                                                & 0.048                                                               & 0.384             & 0.491             & 0.446            & 0.322               & 0.543              & 0.474              & 0.441           & 0.503           \\
                              &                       & Replicate                                                        & 0.020          & 0.023          & 0.058                                                                & 0.040                                                               & 0.467             & 0.494             & 0.457            & 0.492               & 0.579              & 0.617              & 0.483           & 0.555           \\
                              &                       & Circular                                                         & \textbf{0.018} & \textbf{0.021} & \textbf{0.021}                                                       & \textbf{0.020}                                                      & 0.981             & 0.998             & 0.994            & 0.999               & 0.995              & 1.010              & 0.662           & 0.994           \\ \cline{2-15} 
                              & \multirow{4}{*}{$\mathcal{L}_{norm}$} & CPE                                                              & 0.202          & 0.167          & \textbf{0.215}                                                       & \textbf{0.210}                                                      & \textbf{0.221}    & \textbf{0.210}    & \textbf{0.217}   & \textbf{0.222}      & \textbf{0.236}     & \textbf{0.208}     & 0.231           & \textbf{0.220}  \\
                              &                       & Zero                                                             & 0.214          & 0.169          & 0.411                                                                & 0.372                                                               & 0.423             & 0.283             & 0.254            & 0.364               & 0.254              & 0.228              & 0.255           & 0.340           \\
                              &                       & Replicate                                                        & \textbf{0.185} & 0.169          & 0.410                                                                & 0.444                                                               & 0.408             & 0.317             & 0.329            & 0.533               & 0.279              & 0.295              & 0.287           & 0.329           \\
                              &                       & Circular                                                         & 0.196          & \textbf{0.139} & 0.555                                                                & 0.540                                                               & 0.634             & 0.634             & 0.518            & 0.926               & 0.839              & 0.915              & \textbf{0.181}  & 0.798         \\
\bottomrule
\end{tabular}
}
\caption{Quantitative comparison of DyNCA baselines with different padding strategies with the proposed DyNCA model with Cartesian Positional Encoding (CPE). We observe that DyNCA with CPE can better fit most target motions.}
\label{tab:motion-vec-ablation-quantitative}
\end{table*}

\subsection{Motion from Video}
\label{suppsec:cpe-abl}

\subsubsection{Qualitative Analysis}
Without positional encoding, we observe several failed or distorted synthesized video frames, as shown in Figure \ref{fig:cpe-abl-vid}. Training without CPE can cause artifacts on synthesized frames and can lead to texture-less images of low quality.

\newcommand{\imgmvidcpevidabl}[1]{\includegraphics[height=70pt]{Supp/figures/MotionVidCPEAbl/#1}}

\newcolumntype{S}{>{\centering\arraybackslash} m{60pt} } 
\newcolumntype{Q}{>{\centering\arraybackslash} m{2pt} } 
\begin{table}[t]
\resizebox{\linewidth}{!}{
\begin{tabular}{m{2pt}SSSS}
    
% \toprule
    % \textbf{Target} &
    % \textbf{Single-scale} &
    % \textbf{Multi-scale} \\
    
    % \midrule
    
{\rotatebox{90}{\parbox{2.5cm}{\hspace{19pt} \textbf{Target}}}} &
\imgmvidcpevidabl{flames.jpg}                                & \imgmvidcpevidabl{ink.jpg}       & 
 \imgmvidcpevidabl{coral.jpg}  &      
 \imgmvidcpevidabl{lava.jpg} \\

% \midrule  

{\rotatebox{90}{\parbox{2.5cm}{\hspace{20pt} \textbf{Plain}}}} &
                          \imgmvidcpevidabl{flames_noCPE.png}      & \imgmvidcpevidabl{ink_noCPE.png}      &     \imgmvidcpevidabl{coral_noCPE.png}   &    \imgmvidcpevidabl{lava_noCPE.png}                \\
                            {\rotatebox{90}{\parbox{2.5cm}{\hspace{20pt} \textbf{CPE}}}} &
                           \imgmvidcpevidabl{flames_CPE.png} & \imgmvidcpevidabl{ink_CPE.png}     & \imgmvidcpevidabl{coral_CPE.png}      &     \imgmvidcpevidabl{lava_CPE.png}         
                            \\

\end{tabular}
}
\vspace{-10pt}
\captionof{figure}{Comparison between training with and without Cartesian Positional Encoding (CPE). The first row shows the target appearance texture. The results without CPE (second row) have less texture and more artifacts compared with the third row (with CPE). The results are obtained with DyNCA-S-256.}
\label{fig:cpe-abl-vid}
% \vspace{-10pt}
\end{table}

\subsubsection{Quantitative Analysis}

In Table~\ref{tab:pos-emb-abl-loss}, we record the loss values during video synthesis obtained from DyNCA trained with and without Cartesian Positional Encoding(CPE). The method for obtaining $\mathcal{L}_{appr}$ and $\mathcal{L}_{mvid}$ is the same as in the quantitative evaluation of the multi-scale perception ablation study, namely average across all ground-truth frames.

\begin{table}[htbp]
\begin{tabular}{c||cc||cc}
\toprule
\multirow{2}{*}{\begin{tabular}[c]{@{}c@{}}NCA \\ Configs\end{tabular}} & \multicolumn{2}{c||}{$\mathcal{L}_{appr}$}           & \multicolumn{2}{c}{$\mathcal{L}_{mvid}$}           \\ 
                                                                          & \multicolumn{1}{c}{CPE}  & Plain & \multicolumn{1}{c}{CPE}  & Plain \\ \midrule
                    \midrule
DyNCA-S-128                                                               & \multicolumn{1}{c}{\textbf{3.1762}} & {4.3809} & \multicolumn{1}{c}{\textbf{0.1670}} & 0.1874 \\ 
DyNCA-L-128                                                               & \multicolumn{1}{c}{\textbf{3.1789}} & 3.9818 & \multicolumn{1}{c}{\textbf{0.1654}} & 0.1834 \\ 
DyNCA-S-256                                                               & \multicolumn{1}{c}{\textbf{2.5536}} & 2.9358 & \multicolumn{1}{c}{\textbf{0.1959}} & 0.2102 \\ 
DyNCA-L-256                                                               & \multicolumn{1}{c}{\textbf{2.5633}} & 2.8756 & \multicolumn{1}{c}{\textbf{0.1901}} & 0.1980 \\ 
\bottomrule
\end{tabular}
\caption{Loss values during video synthesis after training. "Plain" refers to not adding positional encoding to cell states. CPE contributes to a better fitting of target appearance and motion.}
\label{tab:pos-emb-abl-loss}
\end{table}

In all DyNCA settings, positional encoding helps decrease the test loss during video synthesis, indicating the importance of our proposed positional encoding method.
