# Supplementary material for: DyNCA: Real-time Dynamic Texture Synthesis Using Neural Cellular Automata
Source: arXiv:2211.11417 source file (2023-03-30)
Supplement: Supplementary file 2 [file CompareMethod.tex]

% \section{Implementation of the Two Compared Methods for Video Motion}
% \label{suppsec:compare-method}
% The two compared methods in our experiment section, namely Tesfaldet et al.\cite{two_stream} and Xie et al.\cite{xie2017generativeconvnet}, run experiments on a single TITAN-XP GPU. For a fair comparison of speed between our method and theirs, we re-implement these two methods in PyTorch and test them on a single A100 GPU. Note that we only use the re-implementation for speed tests but still use the public code of their methods for synthesizing videos and performing other evaluations (\href{https://github.com/tesfaldet/two-stream-dyntex-synth}{Tesfaldet et al.\cite{two_stream}}, \href{https://github.com/zilongzheng/STGConvNet}{Xie et al.\cite{xie2017generativeconvnet}}). We find that our PyTorch implementation of the method of Tesfaldet et al.\cite{two_stream} is slower than their original TensorFlow implementation but the training converges much faster. Therefore, we train their method for 1000 epochs instead of 6000 epochs as in the original code and keep everything else the same. For the method of Xie et al.\cite{xie2017generativeconvnet}, we ensure that the number of trainable parameters is the same as in their public code and train ST and FC configurations both for 500 epochs.  
