# Supplementary material for: DyNCA: Real-time Dynamic Texture Synthesis Using Neural Cellular Automata
Source: arXiv:2211.11417 source file (2023-03-30)
Supplement: Supplementary file 3 [file Demo.tex]

\section{Demo}
Our demo is built on top of the open-source demo provided by Niklasson et al. \cite{niklasson2021self-sothtml} in their Self-Organizing Textures paper. Niklasson et al. implement the NCA model using Javascript and WebGL frameworks. We implement DyNCA by building on top of their codebase. Figure~\ref{fig:demo_vector_field} and  \ref{fig:demo_video} show screenshots of our real-time interactive demo available at \href{https://dynca.github.io}{https://dynca.github.io}. We also provide the synthesized videos for our Dynamic Style Transfer experiments at \href{https://dynca.github.io/#style_transfer}{https://dynca.github.io/\#style\_transfer}. 

Besides the screenshots of our demo, we benchmark the performance of the WebGL demo on various devices, including computers and smartphones, and show that DyNCA can synthesize dynamic video textures in real time on low-end GPUs.

\subsection{Qualitative Results}

\textbf{Demo Type: Vector Field Motion:} Figure~\ref{fig:demo_vector_field} shows the demo of DyNCA models that are trained with vector field supervision. The users can choose the desired target vector field and target appearance, and our demo will synthesize the video in real time. The discussed real-time editing controls including \textit{Speed Control}, \textit{Direction Control}, \textit{Editing Brush}, and \textit{Local Coordinate Transformation} are also shown in Figure~\ref{fig:demo_vector_field}. The users can click on the canvas to edit the synthesized video using the brush tool. Our demo also allows the users to control the resolution by the resolution sliders. The resolution control simply changes the spatial dimensions of the seed $H$ and $W$ and re-runs the DyNCA model. The DyNCA models provided in \textit{Vector Field Motion Demo} are trained without \textit{Multi-Scale Perception} and with a seed size of $128 \times 128$. The users can also choose between the DyNCA-S and DyNCA-L configurations.

\textbf{Demo Type: Video Motion:}
Figure~\ref{fig:demo_video} shows a screenshot of the DyNCA demo with models trained with video supervision. The users can choose the desired video used to train the DyNCA model. Here, we train the DyNCA models with \textit{Multi-Scale Perception} enabled and a seed size of $256 \times 256$. The users can also choose between the DyNCA-S and DyNCA-L configurations.

\subsection{Quantitative Results}
For benchmarking the performance of our real-time DyNCA demo, we run the model for 500 steps to calculate the statistics of steps-per-second, frames-per-second (FPS), and how many milliseconds it takes for generating one frame. We show the results for various devices including computers and smartphones in Table \ref{tab:performance-vec} and \ref{tab:performance-vid}. 
Table \ref{tab:performance-vec} summarizes the vector field motion performance when we map 24 NCA steps to one frame, and Table \ref{tab:performance-vid} the video motion when we map 64 NCA steps to one frame. The models trained for video motion are slightly slower because of utilizing multi-scale perception.

\begin{figure*}[ht!]
    \centering
    \includegraphics[width=\linewidth]{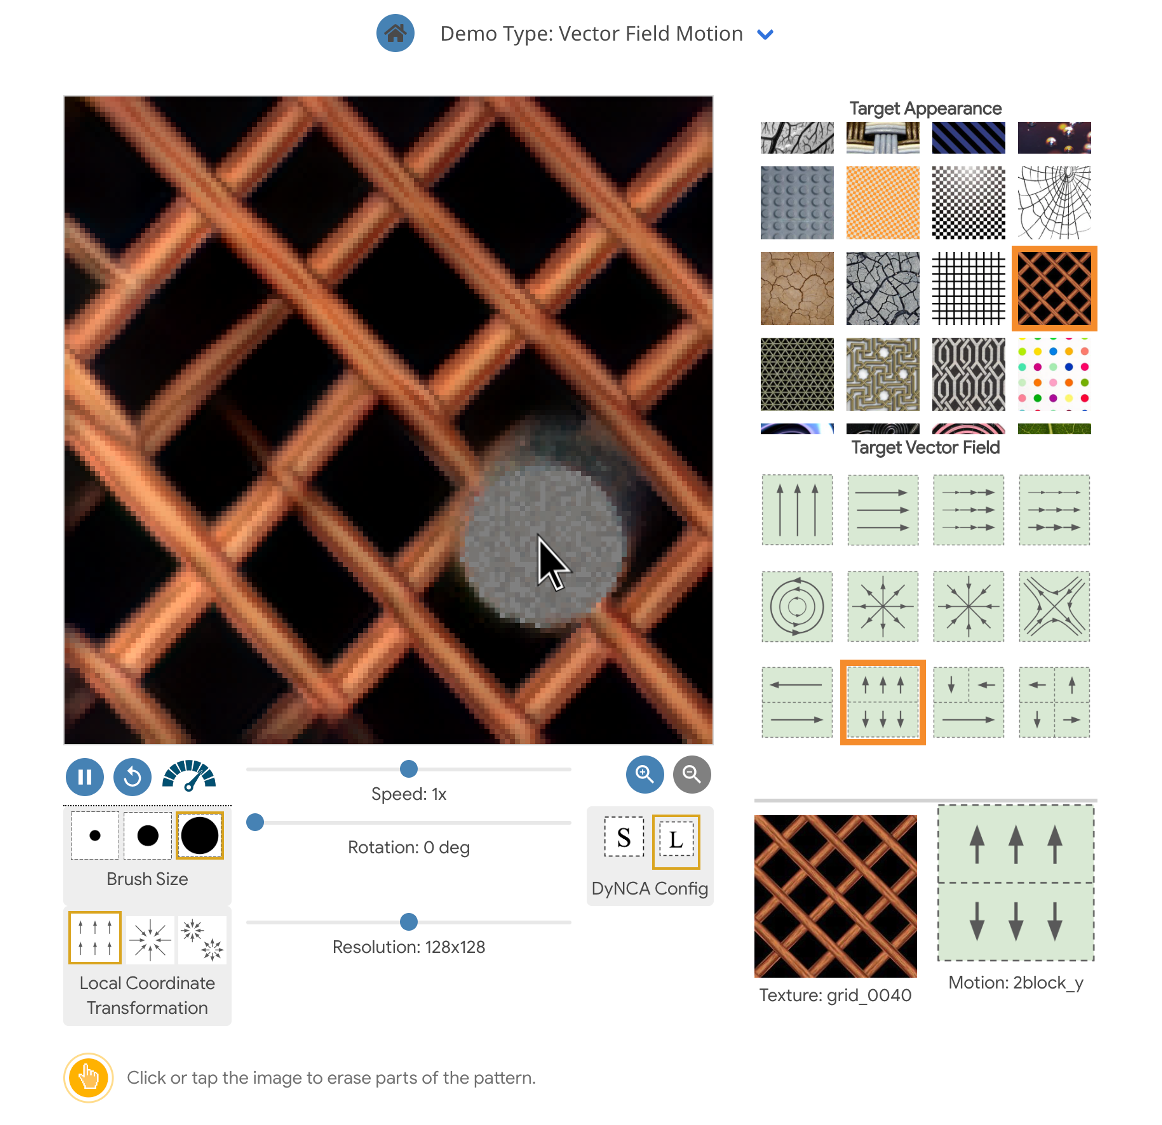}
    \caption{A screenshot for our demo on vector field motion. Users can choose from 45 different target appearance images and 12 different target vector fields, 2 different DyNCA configurations, and  3 different local coordinate transformations. }
    \label{fig:demo_vector_field}
\end{figure*}

\begin{figure*}[ht!]
    \centering
    \includegraphics[width=\linewidth]{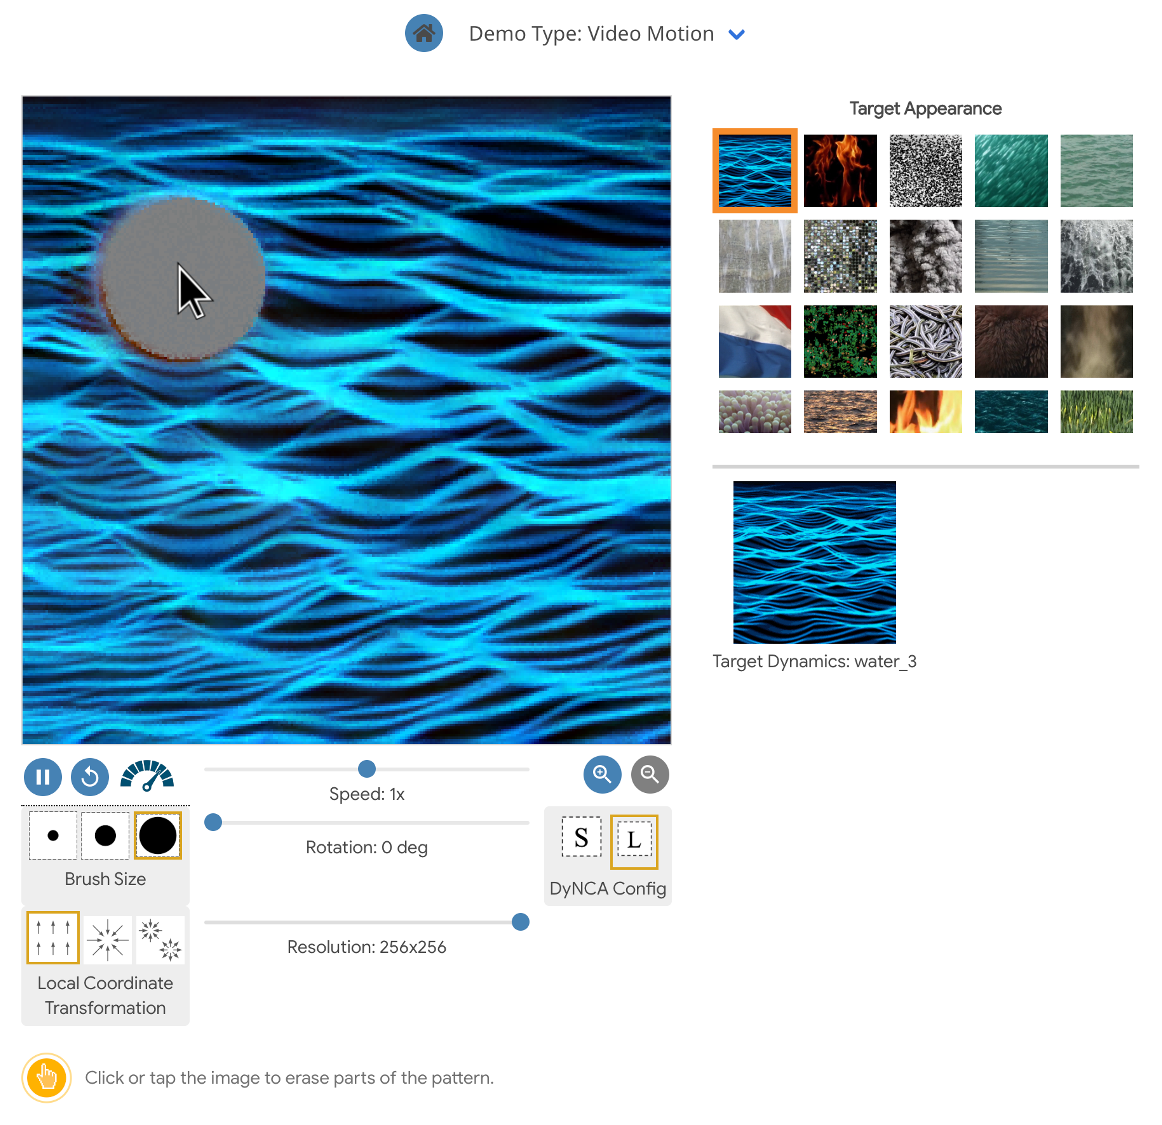}
    \caption{A screenshot for our demo on video motion. Users can choose from 59 different target videos, 2 different DyNCA configurations, and  3 different local coordinate transformations.}
    \label{fig:demo_video}
\end{figure*}

\begin{table*}[ht!]
\centering
\resizebox{\linewidth}{!}{
\begin{tabular}{c||ccS[table-format=5.0]S[table-format=3.2]S[table-format=3.2]}
\textbf{Device name-CPU-GPU}                  & \textbf{\begin{tabular}[c]{@{}c@{}}DyNCA \\ Config\end{tabular}} & \textbf{Seed Size}     & \textbf{steps/s} $\uparrow$ & \textbf{FPS} $\uparrow$ & \textbf{ms/step} $\downarrow$ \\
\midrule
\midrule
\multirow{4}{*}{\begin{tabular}[c]{@{}c@{}} Desktop Computer \\ AMD Ryzen 3970X \\ NVIDIA GeForce RTX 3090 \end{tabular}} & \multirow{2}{*}{S}  & $128 \times 128$ &       14286       &     595.24        &        0.07         \\
                                 &                    & $256 \times 256$  & 4717 & 196.54&  0.21               \\ \cline{2-6} 

 & \multirow{2}{*}{L}  & $128 \times 128$  &10000               & 416.67            & 0.10       \\
                                 &                     & $256 \times 256$ & 2688               & 112.01            & 0.37                \\ 
\midrule
\midrule

\multirow{4}{*}{\begin{tabular}[c]{@{}c@{}} MacBook Pro (16-inch, 2021) \\ Chip Apple M1 Pro \end{tabular}} & \multirow{2}{*}{S}  & $128 \times 128$ &       2747       &     114.47        &        0.36         \\
                                 &                    & $256 \times 256$  & 879 & 36.61&  1.14               \\ \cline{2-6} 

 & \multirow{2}{*}{L}  & $128 \times 128$  &1838               & 76.59            & 0.54       \\
                                 &                     & $256 \times 256$ & 569               & 23.70            & 1.76                \\ 
\midrule
\midrule

\multirow{4}{*}{\begin{tabular}[c]{@{}c@{}} Terrans Force X711 PLUS 67SH1 \\ Intel(R) Core(TM) i7-6700K \\ GTX 980M GPU\end{tabular}} & \multirow{2}{*}{S}  & $128 \times 128$ &       2212       &     92.18        &        0.45         \\
                                 &                    & $256 \times 256$  & 484 & 20.17&  2.07               \\ \cline{2-6} 

 & \multirow{2}{*}{L}  & $128 \times 128$  &1381               & 57.55            & 0.72       \\
                                 &                     & $256 \times 256$ & 303               & 12.64            & 3.30                \\ 
\midrule
\midrule

\multirow{4}{*}{\begin{tabular}[c]{@{}c@{}} MacBook Pro (13-inch, 2020) \\ 2.3 GHz Quad-Core Intel Core i7 \\ Intel Iris Plus Graphics 1536 MB\end{tabular}} & \multirow{2}{*}{S}  & $128 \times 128$ &       1299       &     54.11       &        0.77        \\

                                 &                    & $256 \times 256$  & 247 & 10.28&  4.05               \\ \cline{2-6} 

 & \multirow{2}{*}{L}  & $128 \times 128$  & 818               & 34.10            & 1.22       \\
                                 &                     & $256 \times 256$ & 160               & 6.67            & 6.25                \\ 
\midrule
\midrule
% \multirow{4}{*}{\begin{tabular}[c]{@{}c@{}} Matebook X Pro \\ Intel(R) Core(TM) i7-10510U \\ MX250 GPU\end{tabular}} & \multirow{2}{*}{S}  & $128 \times 128$ &       486       &     20.27        &        2.06         \\
%                                  &                    & $256 \times 256$  & 121 & 5.04 &  8.27               \\ \cline{2-6} 

%  & \multirow{2}{*}{L}  & $128 \times 128$  &312               & 13.02            & 3.20       \\
%                                  &                     & $256 \times 256$ & 73               & 3.06            & 13.62                \\ 
% \midrule
% \midrule

% \multirow{4}{*}{\begin{tabular}[c]{@{}c@{}} EP's-Phone\end{tabular}} & \multirow{2}{*}{S}  & $128 \times 128$ &       step       &     fps        &        ms         \\
%                                  &                    & $256 \times 256$  & step & fps&  ms               \\ \cline{2-6} 

%  & \multirow{2}{*}{L}  & $128 \times 128$  &step               & fps            & ms       \\
%                                  &                     & $256 \times 256$ & step               & fps            & ms                \\ 
% \midrule
% \midrule

\multirow{4}{*}{\begin{tabular}[c]{@{}c@{}} Apple iPhone 14 \\ Hexa-core Apple GPU (5-core graphics)\end{tabular}} & \multirow{2}{*}{S}  & $128 \times 128$ &       1037       &     43.22        &        0.96         \\
                                 &                    & $256 \times 256$  & 217 & 9.06&  4.60               \\ \cline{2-6} 

 & \multirow{2}{*}{L}  & $128 \times 128$  &643               & 26.78            & 1.56       \\
                                 &                     & $256 \times 256$ & 130               & 5.42            & 7.69                \\ 
\midrule
\midrule

\multirow{4}{*}{\begin{tabular}[c]{@{}c@{}} Samsung Galaxy Z Flip4 \\ Octa-core CPU Adreno 730 GPU \end{tabular}} & \multirow{2}{*}{S}  & $128 \times 128$ &       1029       &     42.87        &        0.97         \\
                                 &                    & $256 \times 256$  & 223 & 9.30&  4.48               \\ \cline{2-6} 

 & \multirow{2}{*}{L}  & $128 \times 128$  &608               & 25.34            & 1.64       \\
                                 &                     & $256 \times 256$ & 141               & 5.88            & 7.09                \\ 
\midrule
\midrule

\multirow{4}{*}{\begin{tabular}[c]{@{}c@{}} iPad Air (4th generation) \\ A14 Bionic chip \end{tabular}} & \multirow{2}{*}{S}  & $128 \times 128$ &       697       &     29.06        &        1.43         \\
                                 &                    & $256 \times 256$  & 139 & 5.78&  7.21               \\ \cline{2-6} 

 & \multirow{2}{*}{L}  & $128 \times 128$  &450               & 18.75            & 2.22       \\
                                 &                     & $256 \times 256$ & 93               & 3.87            & 10.76                \\ 
\midrule
\midrule

\multirow{4}{*}{\begin{tabular}[c]{@{}c@{}} Apple iPhone 12 \\ A14 Bionic chip \end{tabular}} & \multirow{2}{*}{S}  & $128 \times 128$ &       717       &     29.89        &        1.39         \\
                                 &                    & $256 \times 256$  & 162 & 6.74&  6.18               \\ \cline{2-6} 

 & \multirow{2}{*}{L}  & $128 \times 128$  &457               & 19.04            & 2.19       \\
                                 &                     & $256 \times 256$ & 101               & 4.23            & 9.84                \\ 
\midrule
\midrule

\end{tabular}
}
\caption{Benchmark of DyNCA WebGL implementations on different devices. This table shows the results for the Demo Type \textit{Vector Field Motion}. In this configuration we set $T=24$, i.e. we map 24 DyNCA steps to one video frame.  }
\label{tab:performance-vec}
% }
\end{table*}

\begin{table*}[ht!]
\resizebox{\linewidth}{!}{
\begin{tabular}{c||ccS[table-format=5.0]S[table-format=3.2]S[table-format=3.2]}
\textbf{Device name-CPU-GPU}                  & \textbf{\begin{tabular}[c]{@{}c@{}}DyNCA \\ Config\end{tabular}} & \textbf{Seed Size}     & \textbf{steps/s} $\uparrow$ & \textbf{FPS} $\uparrow$ & \textbf{ms/step} $\downarrow$ \\
\midrule
\midrule
\multirow{4}{*}{\begin{tabular}[c]{@{}c@{}} Desktop Computer \\ AMD Ryzen 3970X \\ NVIDIA GeForce RTX 3090 \end{tabular}} & \multirow{2}{*}{S}  & $128 \times 128$ &       10638       &     166.22        &        0.09         \\
                                 &                    & $256 \times 256$  & 2688 & 42.00&  0.37               \\ \cline{2-6} 

 & \multirow{2}{*}{L}  & $128 \times 128$  &8065               & 126.01            & 0.12       \\
                                 &                     & $256 \times 256$ & 2415               & 37.74            & 0.41                \\ 
\midrule
\midrule

\multirow{4}{*}{\begin{tabular}[c]{@{}c@{}} MacBook Pro (16-inch, 2021) \\ Chip Apple M1 Pro \end{tabular}} & \multirow{2}{*}{S}  & $128 \times 128$ &       2326       &     35.34        &        0.43         \\
                                 &                    & $256 \times 256$  & 761 & 11.89&  1.31               \\ \cline{2-6} 

 & \multirow{2}{*}{L}  & $128 \times 128$  &1602               & 25.04            & 0.62       \\
                                 &                     & $256 \times 256$ & 508               & 7.93            & 1.97                \\ 
\midrule
\midrule

\multirow{4}{*}{\begin{tabular}[c]{@{}c@{}} Terrans Force X711 PLUS 67SH1 \\ Intel(R) Core(TM) i7-6700K \\
GTX 980M GPU\end{tabular}} & \multirow{2}{*}{S}  & $128 \times 128$ &       1923       &     30.05        &        0.52         \\
                                 &                    & $256 \times 256$  & 437 & 6.83&  2.29               \\ \cline{2-6} 

 & \multirow{2}{*}{L}  & $128 \times 128$  &1225               & 19.15            & 0.82       \\
                                 &                     & $256 \times 256$ & 278               & 4.35            & 3.59                \\ 
\midrule
\midrule

\multirow{4}{*}{\begin{tabular}[c]{@{}c@{}} MacBook Pro (13-inch, 2020) \\ 2.3 GHz Quad-Core Intel Core i7 \\ Intel Iris Plus Graphics 1536 MB\end{tabular}} & \multirow{2}{*}{S}  & $128 \times 128$ &       1055       &     16.48       &        0.95        \\

                                 &                    & $256 \times 256$  & 214 & 3.35&  4.66               \\ \cline{2-6} 

 & \multirow{2}{*}{L}  & $128 \times 128$  & 682               & 10.66            & 1.47       \\
                                 &                     & $256 \times 256$ & 139               & 2.17        & 7.20                \\ 
\midrule
\midrule

% \multirow{4}{*}{\begin{tabular}[c]{@{}c@{}} Matebook X Pro \\ Intel(R) Core(TM) i7-10510U \\ MX250 GPU\end{tabular}} & \multirow{2}{*}{S}  & $128 \times 128$ &       442       &     6.91        &        2.26         \\
%                                  &                    & $256 \times 256$  & 283 & 4.43 &  3.53               \\ \cline{2-6} 

%  & \multirow{2}{*}{L}  & $128 \times 128$  &108               & 1.69            & 9.26       \\
%                                  &                     & $256 \times 256$ & 65               & 1.03            & 15.21                \\ 
% \midrule
% \midrule

% \multirow{4}{*}{\begin{tabular}[c]{@{}c@{}} EP's-Phone\end{tabular}} & \multirow{2}{*}{S}  & $128 \times 128$ &       step       &     fps        &        ms         \\
%                                  &                    & $256 \times 256$  & step & fps&  ms               \\ \cline{2-6} 

%  & \multirow{2}{*}{L}  & $128 \times 128$  &step               & fps            & ms       \\
%                                  &                     & $256 \times 256$ & step               & fps            & ms                \\ 

% \midrule
% \midrule

\multirow{4}{*}{\begin{tabular}[c]{@{}c@{}} Apple iPhone 14 \\ Hexa-core Apple GPU (5-core graphics)\end{tabular}} & \multirow{2}{*}{S}  & $128 \times 128$ &       929       &     14.52        &        1.08         \\
                                 &                    & $256 \times 256$  & 191 & 2.98&  5.24               \\ \cline{2-6} 

 & \multirow{2}{*}{L}  & $128 \times 128$  &597               & 9.32            & 1.68       \\
                                 &                     & $256 \times 256$ & 117               & 1.82            & 8.57               \\ 

\midrule
\midrule

\multirow{4}{*}{\begin{tabular}[c]{@{}c@{}} Samsung Galaxy Z Flip4 \\ Octa-core CPU Adreno 730 GPU
\end{tabular}} & \multirow{2}{*}{S}  & $128 \times 128$ &       873       &     13.63        &        1.15         \\
                                 &                    & $256 \times 256$  & 207 & 3.23&  4.84               \\ \cline{2-6} 

 & \multirow{2}{*}{L}  & $128 \times 128$  &557               & 3.96            & 3.94       \\
                                 &                     & $256 \times 256$ & 129               & 2.02            & 7.74                \\ 
\midrule
\midrule

\multirow{4}{*}{\begin{tabular}[c]{@{}c@{}} iPad Air (4th generation) \\ A14 Bionic chip\end{tabular}} & \multirow{2}{*}{S}  & $128 \times 128$ &       600       &     9.37        &        1.67         \\
                                 &                    & $256 \times 256$  & 134 & 2.09&  7.48               \\ \cline{2-6} 

 & \multirow{2}{*}{L}  & $128 \times 128$  &412               & 8.70            & 1.80       \\
                                 &                     &  $256 \times 256$ & 85               & 1.33            & 11.79                \\ 
\midrule
\midrule

\multirow{4}{*}{\begin{tabular}[c]{@{}c@{}} Apple iPhone 12 \\ A14 Bionic chip \end{tabular}} & \multirow{2}{*}{S}  & $128 \times 128$ &       598       &    0.36        &        1.67         \\
                                 &                    & $256 \times 256$  & 144 & 2.26&  6.92               \\ \cline{2-6} 

 & \multirow{2}{*}{L}  & $128 \times 128$  &418               & 6.54          & 2.39       \\
                                 &                     & $256 \times 256$ & 92               & 1.43           & 10.89                \\ 
\midrule
\midrule

\end{tabular}
}
\caption{Benchmark of DyNCA WebGL implementations on different devices. This table shows the results for the Demo Type \textit{Video Motion}. In this configuration multi-scale perception is enabled, and we set $T=64$, i.e., we map 64 DyNCA steps to one video frame. }
\label{tab:performance-vid}
\end{table*}

\clearpage
\newpage
