# Supplementary material for: DyNCA: Real-time Dynamic Texture Synthesis Using Neural Cellular Automata
Source: arXiv:2211.11417 source file (2023-03-30)
Supplement: Supplementary file 4 [file MotionVidDST.tex]

\begin{table*}[]
\begin{tabular}{F|Gm{0pt}G|||Gm{0pt}G}

    {\multirow{2}{*}{\textbf{Target Appearance}}} & \multicolumn{3}{c|||}{\hspace{-8pt}\textbf{Target Dynamics (Motion)}} & \multicolumn{3}{c}{\hspace{-4pt}\textbf{Synthesized Result}} \\
    
    \vspace{18pt}

                                       & Video     &        & Optical Flow     & Video      &        & Optical Flow     \\
    \midrule

 \imgmvidsupp{water_3-cartoon_water_4.png}& \imgmvidsupp{water_3-cartoon_water_4_target.png} &\ofarrow& \imgmvidsupp{water_3-cartoon_water_4_targetflow.png}& \imgmvidsupp{water_3-cartoon_water_4_gen.png} & \ofarrow& \imgmvidsupp{water_3-cartoon_water_4_genflow.png}\\
 \imgmvidsupp{fireplace_2-cartoon_fire_6.png}& \imgmvidsupp{fireplace_2-cartoon_fire_6_target.png} &\ofarrow& \imgmvidsupp{fireplace_2-cartoon_fire_6_targetflow.png}& \imgmvidsupp{fireplace_2-cartoon_fire_6_gen.png} & \ofarrow& \imgmvidsupp{fireplace_2-cartoon_fire_6_genflow.png}\\
 \imgmvidsupp{sea_2-cartoon_water_4.png}& \imgmvidsupp{sea_2-cartoon_water_4_target.png} &\ofarrow& \imgmvidsupp{sea_2-cartoon_water_4_targetflow.png}& \imgmvidsupp{sea_2-cartoon_water_4_gen.png} & \ofarrow& \imgmvidsupp{sea_2-cartoon_water_4_genflow.png}\\
 \imgmvidsupp{fireplace_2-cartoon_fire_3.png}& \imgmvidsupp{fireplace_2-cartoon_fire_3_target.png} &\ofarrow& \imgmvidsupp{fireplace_2-cartoon_fire_3_targetflow.png}& \imgmvidsupp{fireplace_2-cartoon_fire_3_gen.png} & \ofarrow& \imgmvidsupp{fireplace_2-cartoon_fire_3_genflow.png}\\
 \imgmvidsupp{flames-cartoon_fire_6.png}& \imgmvidsupp{flames-cartoon_fire_6_target.png} &\ofarrow& \imgmvidsupp{flames-cartoon_fire_6_targetflow.png}& \imgmvidsupp{flames-cartoon_fire_6_gen.png} & \ofarrow& \imgmvidsupp{flames-cartoon_fire_6_genflow.png}\\
 \imgmvidsupp{fireplace_1-cartoon_fire_4.png}& \imgmvidsupp{fireplace_1-cartoon_fire_4_target.png} &\ofarrow& \imgmvidsupp{fireplace_1-cartoon_fire_4_targetflow.png}& \imgmvidsupp{fireplace_1-cartoon_fire_4_gen.png} & \ofarrow& \imgmvidsupp{fireplace_1-cartoon_fire_4_genflow.png}\\
 \imgmvidsupp{water_3-cartoon_water_1.png}& \imgmvidsupp{water_3-cartoon_water_1_target.png} &\ofarrow& \imgmvidsupp{water_3-cartoon_water_1_targetflow.png}& \imgmvidsupp{water_3-cartoon_water_1_gen.png} & \ofarrow& \imgmvidsupp{water_3-cartoon_water_1_genflow.png}\\

\end{tabular}
\captionof{figure}{Results of dynamic style transfer with DyNCA-L-256. }
\label{tab:video-result-dst-more1}
\end{table*}
