# Supplementary material for: DyNCA: Real-time Dynamic Texture Synthesis Using Neural Cellular Automata
Source: arXiv:2211.11417 source file (2023-03-30)
Supplement: Supplementary file 5 [file MotionVidResMore.tex]

% Please add the following required packages to your document preamble:
% \usepackage{multirow}

\newcommand{\imgmvidsupp}[1]{\includegraphics[height=75pt]{Supp/figures/MotionVid/#1}}

\newcolumntype{G}{>{\centering\arraybackslash} m{75pt} }  %# New column type
\newcolumntype{F}{>{\centering\arraybackslash} m{80pt} } 
\newcolumntype{H}{>{\centering\arraybackslash} m{5pt} }  %# New column type
%# New column type

\begin{table*}[]
\begin{tabular}{F|Gm{0pt}G|||Gm{0pt}G}

    {\multirow{2}{*}{\textbf{Target Appearance}}} & \multicolumn{3}{c|||}{\hspace{-8pt}\textbf{Target Dynamics (Motion)}} & \multicolumn{3}{c}{\hspace{-4pt}\textbf{Synthesized Result}} \\
    
    \vspace{18pt}

                                       & Video     &        & Optical Flow     & Video      &        & Optical Flow     \\
    \midrule

\imgmvidsupp{fur.png}& \imgmvidsupp{fur_target.png} &\ofarrow& \imgmvidsupp{fur_targetflow.png}& \imgmvidsupp{fur_gen.png} & \ofarrow& \imgmvidsupp{fur_genflow.png}\\
 \imgmvidsupp{candy_1.png}& \imgmvidsupp{candy_1_target.png} &\ofarrow& \imgmvidsupp{candy_1_targetflow.png}& \imgmvidsupp{candy_1_gen.png} & \ofarrow& \imgmvidsupp{candy_1_genflow.png}\\
 \imgmvidsupp{sea_4.png}& \imgmvidsupp{sea_4_target.png} &\ofarrow& \imgmvidsupp{sea_4_targetflow.png}& \imgmvidsupp{sea_4_gen.png} & \ofarrow& \imgmvidsupp{sea_4_genflow.png}\\
 \imgmvidsupp{shiny_circles.png}& \imgmvidsupp{shiny_circles_target.png} &\ofarrow& \imgmvidsupp{shiny_circles_targetflow.png}& \imgmvidsupp{shiny_circles_gen.png} & \ofarrow& \imgmvidsupp{shiny_circles_genflow.png}\\
 \imgmvidsupp{plants.png}& \imgmvidsupp{plants_target.png} &\ofarrow& \imgmvidsupp{plants_targetflow.png}& \imgmvidsupp{plants_gen.png} & \ofarrow& \imgmvidsupp{plants_genflow.png}\\
 \imgmvidsupp{calm_water_6.png}& \imgmvidsupp{calm_water_6_target.png} &\ofarrow& \imgmvidsupp{calm_water_6_targetflow.png}& \imgmvidsupp{calm_water_6_gen.png} & \ofarrow& \imgmvidsupp{calm_water_6_genflow.png}\\
 \imgmvidsupp{underwater_vegetation_1.png}& \imgmvidsupp{underwater_vegetation_1_target.png} &\ofarrow& \imgmvidsupp{underwater_vegetation_1_targetflow.png}& \imgmvidsupp{underwater_vegetation_1_gen.png} & \ofarrow& \imgmvidsupp{underwater_vegetation_1_genflow.png}\\

\end{tabular}
\captionof{figure}{Results of dynamic texture synthesis with DyNCA-L-256. }
\label{tab:video-result-more1}
\end{table*}
