# Supplementary material for: DyNCA: Real-time Dynamic Texture Synthesis Using Neural Cellular Automata
Source: arXiv:2211.11417 source file (2023-03-30)
Supplement: Supplementary file 6 [file MultiscaleAbl.tex]

\section{Quantitative Evaluation of Multi-scale Perception Ablation Study}
\label{suppsec:multi-scale}
\begin{table}[htbp]
\begin{tabular}{c||cc||cc}
\toprule
\multirow{2}{*}{\begin{tabular}[c]{@{}c@{}}NCA \\ Configs\end{tabular}} & \multicolumn{2}{c||}{$\mathcal{L}_{appr}$}           & \multicolumn{2}{c}{$\mathcal{L}_{mvid}$}           \\ 
                                                                          & \multicolumn{1}{c}{Multi}  & Single & \multicolumn{1}{c}{Multi}  & Single \\ \midrule
                    \midrule
DyNCA-S-128                                                               & \multicolumn{1}{c}{3.1816} & \textbf{3.1762} & \multicolumn{1}{c}{0.1707} & \textbf{0.1670} \\ 
DyNCA-L-128                                                               & \multicolumn{1}{c}{\textbf{3.1267}} & 3.1789 & \multicolumn{1}{c}{\textbf{0.1641}} & 0.1654 \\ 
DyNCA-S-256                                                               & \multicolumn{1}{c}{\textbf{2.5536}} & 2.6343 & \multicolumn{1}{c}{\textbf{0.1959}} & 0.2008 \\ 
DyNCA-L-256                                                               & \multicolumn{1}{c}{\textbf{2.5633}} & 2.6918 & \multicolumn{1}{c}{\textbf{0.1901}} & 0.1979 \\ 
\bottomrule
\end{tabular}
\caption{Loss values during video synthesis after training. Multi-scale perception helps decrease the values of $\mathcal{L}_{appr}$ and $\mathcal{L}_{mvid}$, thus contributing to DyNCA better fitting the target appearance and motion.}
\label{tab:multiscale-abl-loss}
\end{table}

In the main paper, we show qualitative results of the ablation study for multi-scale perception. We further quantitatively evaluate the effect of multi-scale perception by observing $\mathcal{L}_{appr}$ and $\mathcal{L}_{mvid}$ during video synthesis after training. In video synthesis, DyNCA generates one frame every $T$ steps, where $T=64$. Denote two consecutive frames as $\mathcal{I}^g_{t},\mathcal{I}^g_{t+T}$, where $t$ is the current time step. We compute $\mathcal{L}_{appr}$ for $\mathcal{I}^g_{t}$ and all frames in the target video. Then we average the result to obtain $\mathcal{L}^t_{appr}$. The final test $\mathcal{L}_{appr}$ is obtained via averaging over all time steps. We also adopt this scheme for computing $\mathcal{L}_{mvid}$, where the inputs are $\mathcal{I}^g_{t},\mathcal{I}^g_{t+T}$. 

In Table \ref{tab:multiscale-abl-loss}, we can see that multi-scale perception helps decrease the loss values overall. When DyNCA has more parameters and the resolution of seeds is large (DyNCA-L-256), the effect becomes more obvious. 
% \footnotetext{\href{https://dynca.github.io/\#style_transfer}{https://dynca.github.io/\#style\_transfer}}
