# Supplementary material for: DyNCA: Real-time Dynamic Texture Synthesis Using Neural Cellular Automata
Source: arXiv:2211.11417 source file (2023-03-30)
Supplement: Supplementary file 7 [file TrainDetails.tex]

\clearpage
\section{Training Details of DyNCA}
We adopt the checkpoint pool trick introduced in \cite{mordvintsev2020growing}. We use a pool size of 256 and initialize the pool with zero-filled constant tensors as the seed. During training, we select a batch of states from the pool, evolve those states according to the DyNCA update rule, and then put the updated states back in the pool. Using a checkpoint pool allows the DyNCA model to see longer horizons of its PDE update rule, and helps with the long-term stability of the DyNCA evolution. Once every 8 epochs we replace one of the states in the pool with the initial seed state. This helps DyNCA to remember the seed state as the initial state of the PDE. 

 We also use the overflow loss introduced in \cite{mordvintsev2020growing, niklasson2021self-sothtml} to ensure training stability. Given a cell state of DyNCA $\mathbf{S}^{t} \in \mathbb{R}^{H \times W \times C}$, the overflow loss  $\mathcal{L}_{over}$ of $\mathbf{S}$ is defined as:
% \begin{equation}
%     \mathcal{L}_{over} = \frac{1}{HWC} \sum^{W}_{i} \sum^{H}_{j} \sum^{C}_{c} \left ( |S_{i,j,c}| - min(|S_{i,j,c}|, 1.0) \right)
% \label{eq:overflow-loss1}
% \end{equation},

$$\mathcal{L}_{over} = \frac{1}{HWC} \sum^{W}_{i} \sum^{H}_{j} \sum^{C}_{c} \left |\mathbf{S}^{t}_{i,j,c} - clip_{[-1,1]} (\mathbf{S}^{t}_{i,j,c}) \right |$$ 
\begin{equation}
    \quad \quad \quad clip_{[a,b]} (x) = max(a, min(x,b)), \; \; \; \; \; \; \; \; \; \; \;
\label{eq:overflow-loss2}
\end{equation}
where $S_{i,j,c}$ is one of the entries of the DyNCA state tensor $\mathbf{S}$. Our final training objective is:
\begin{equation}
    \mathcal{L}_{final} = \mathcal{L}_{\textup{DyNCA}} + c \mathcal{L}_{over},
\label{eq:final-loss}
\end{equation}
where $c$ is the overflow loss weight. Recall that $\mathcal{L}_{\textup{DyNCA}}$, defined in page~4 section~4 of the main paper, consists of the DyNCA objectives for fitting the target appearance and target dynamics. The overflow loss is only computed on the last cell state in one training epoch. 

In addition, we also adopt the gradient normalization trick introduced in \cite{niklasson2021self-sothtml}, and normalize the L2 norm of each layer's gradient before applying them. Gradient normalization stabilizes the training and helps to prevent divergence during training. 
We train for 4000 epochs with an initial learning rate of 0.001, while multiplying the learning rate by 0.3 at 1000 and 2000 epochs.

For the optic flow prediction network, we re-implement the MSOENet introduced in \cite{two_stream} with PyTorch. We use the pre-trained TensorFlow model weights provided by \cite{two_stream} and transfer those weights to our PyTorch model.

In the following sections, we discuss the details of motion-learning training schemes from, first, motion from vector fields and, second, motion from videos.

\subsection{Motion From Vector Field}

For training DyNCA to synthesize motion according to a target vector field, we pick two synthesized images $\mathcal{I}^g_{t_1}, \mathcal{I}^g_{t_2}$ from the synthesized image sequence, and evaluate the loss $\mathcal{L}_{mvec}$ using these two images. Recall our loss functions from Equations~(6, 7, 8) in page 5 of the main paper:
\begin{equation}
\mathcal{L}_{dir} = \frac{1}{HW} \sum_{i, j} \left ( 1 - \frac{U^g_{ij} \cdot U^t_{ij}}{\left \| U^g_{ij} \right \|_2 \left \| U^t_{ij} \right \|_2 } \right ),
\label{eq:dir_loss}
\end{equation}

\begin{equation}
\mathcal{L}_{norm} = \frac{1}{HW} \sum_{i, j}  \left | \frac{T}{t_2 - t_1}\left \| U^g_{ij} \right \|_2 - \left \| U^t_{ij} \right \|_2 \right |.
\label{eq:norm_loss}
\end{equation}

\begin{equation}
\mathcal{L}_{mvec} = \left ( 1.0 - min\{1.0, \mathcal{L}_{dir}\} \right ) \mathcal{L}_{norm} + \gamma \mathcal{L}_{dir},
\label{eq:mvec_loss}
\end{equation}

We use $T = 24$ in our motion from vector field experiments. We set $t_1$ to be the timestep of the selected states from the checkpoint pool and set $t_2 = t_1 + \mathcal{U}(32, 128)$, where $\mathcal{U}(32, 128)$ is a randomly chosen integer between 32 and 128. We use a seed size of $128 \times 128$ and a batch size of 4. We set the direction loss weight $ \gamma = 1.5$, and the overflow loss weight $c = 100.0$. We set the initial motion loss weight to $\lambda=10.0$ and then anneal this weight according to the appearance loss. We find this weight annealing helpful for fitting the motion from a target vector field. 

% be equal the the appearance loss of the first epoch divided by 5.0, and then update the motion loss weight at epoch 500 with the last appearance loss again divided by 5.0. Then, every 500 epochs, we update the motion loss weight to be equal to the median of the appearance losses after the 500 epochs divided by 5.0. \textbf{WHY? IS THIS EMPIRICAL OR DONE BY OTHERS?}

In the next section, we provide the mathematical expressions of the target vector fields we use to train DyNCA.

\subsubsection{Mathematical Expression of Target Vector Fields}

We provide the mathematical definitions of each of the 12 hand-crafted motion vector fields we use to train the DyNCA models. Let $\tilde{U}^t_{i,j}$ be the un-normalized motion vector for each point $(i,j)$ on the vector field image with size $H,W$, where $i \in [-\frac{W}{2},\frac{W}{2}]$ and $j \in [-\frac{H}{2},\frac{H}{2}]$. 
To obtain the final target vector field $U^t$, we L2-normalize $\tilde{U}^t$ using the following equation:
\begin{equation}
 U^t=\frac{\tilde{U}^t}{\frac{1}{HW}\sum_{i,j}||\tilde{U}^t_{i,j}||_{2}}   
\end{equation}

\begin{itemize}
    \item \textbf{Right.} $\tilde{U}^t_{i,j}=(cos(0^\circ),sin(0^\circ))$.
    \item \textbf{Up.} $\tilde{U}^t_{i,j}=(cos(270^\circ),sin(270^\circ))$.
    \item \textbf{Right acc. Right.} $\tilde{U}^t_{i,j}=(\frac{2i+W}{2} \times cos(0^\circ), sin(0^\circ))$.
    \item \textbf{Right acc. Down.} $\tilde{U}^t_{i,j}=(\frac{2j+H}{2} \times cos(0^\circ), sin(0^\circ))$.
    \item \textbf{Circular.}  $\tilde{U}^t_{i,j}=(\frac{j}{\sqrt{H^2 + W^2}},\frac{-i}{\sqrt{H^2 + W^2}})$.
    \item \textbf{Converge.}  $\tilde{U}^t_{i,j}=(\frac{-i}{ \sqrt{i^2 + j^2}},\frac{-j}{ \sqrt{i^2 + j^2}})$.
    \item \textbf{Diverge.} $\tilde{U}^t_{i,j}=(\frac{i}{ \sqrt{i^2 + j^2}},\frac{j}{ \sqrt{i^2 + j^2}})$.
    \item \textbf{Hyperbolic.}  $\tilde{U}^t_{i,j}=(\frac{j}{\sqrt{H^2 + W^2}},\frac{i}{\sqrt{H^2 + W^2}})$.
    \item \textbf{2Block\_X}. 
    \begin{equation}
    % \label{eq2blockx}
    \tilde{U}^t_{i,j}=\left\{
    \begin{aligned}
    (cos(0^\circ),sin(0^\circ)) & , & j \geq 0 , \\
    (cos(180^\circ),sin(180^\circ)) & , & j < 0.
    \end{aligned}
    \right.
    \nonumber
     \end{equation}
    \item \textbf{2Block\_Y}. 
    \begin{equation}
    % \label{eq2blocky}
    \tilde{U}^t_{i,j}=\left\{
    \begin{aligned}
    (cos(90^\circ),sin(90^\circ)) & , & j \geq 0 , \\
    (cos(270^\circ),sin(270^\circ)) & , & j < 0.
    \end{aligned}
    \right.
    \nonumber
    \end{equation}
    
    \item \textbf{3Block}. 
    \begin{equation}
    % \label{eq3block}
    \tilde{U}^t_{i,j}=\left\{
    \begin{aligned}
    (cos(0^\circ),sin(0^\circ)) & , & j \geq 0, \\
    (cos(180^\circ),sin(180^\circ)) & , & i \geq 0, j < 0, \\
    (cos(90^\circ),sin(90^\circ)) & , & i < 0, j < 0.
    \end{aligned}
    \right.
    \nonumber
    \end{equation}
    
    \item \textbf{4Block}. 
    \begin{equation}
    % \label{eq4block}
    \tilde{U}^t_{i,j}=\left\{
    \begin{aligned}
    (cos(0^\circ),sin(0^\circ)) & , & i \geq 0, j \geq 0 \\
    (cos(270^\circ),sin(270^\circ)) & , & i \geq 0,j < 0 \\
    (cos(90^\circ),sin(90^\circ)) & , & i < 0, j \geq 0, \\
    (cos(180^\circ),sin(180^\circ)) & , & i < 0, j < 0.
    \end{aligned}
    \right.
    \nonumber
    \end{equation}
\end{itemize}

\subsection{Motion From Video}

\subsubsection{Dynamic Texture Synthesis}
We use video textures from the dataset introduced in \cite{two_stream}, employing all 12 frames in each video for training. When learning the motion from target videos, DyNCA iterates between 80 and 144 steps at each training epoch. The overflow loss weight $c$ is 1.0.  When training with a seed size of $128 \times 128$, we set the batch size to 4. For training with $256 \times 256$ seed size, we set the batch size to 3 due to GPU memory limits.

% \subsection{Motion Loss Weight Setting}
DyNCA is sensitive to $\lambda$, the weight of the motion loss. Small $\lambda$'s can cause wrong motion or fixed frames while large values can lead to failed texture fitting. To automatically set the weight for motion loss, we first train DyNCA for 1000 epochs with an empirical motion loss weight of 5.0. Then we record the median of the motion loss, denoted as $\mathcal{L}^{median}_{mvid}$, and re-initialize DyNCA and the pool. We find a roughly linear relationship between the median loss and the proper weight and set the weight according to it. We give the concrete values of $\lambda$ for each DyNCA configuration as follows:
\begin{itemize}
    \item S-128, L-128: $ 5.82\times \mathcal{L}^{median}_{mvid} - 1.05$.
    \item S-256, L-256: $ 6.04\times \mathcal{L}^{median}_{mvid} - 2.17$.
\end{itemize}
Finally, we train DyNCA with extra 4000 epochs.

\newcolumntype{S}{>{\centering\arraybackslash} m{60pt} } 
\newcolumntype{Q}{>{\centering\arraybackslash} m{2pt} } 

\subsubsection{Choice of NCA Interval in Video Motion}
When DyNCA learns target motions from videos, it uses $T$ steps to fit one frame of the video. Larger $T$ can contribute to a better fitting of the target motion and appearance since DyNCA acts as a discrete-time PDE and thus more time steps can make the result more precise. We show results with DyNCA intervals of 32 compared to 64, which is what we use in the experiments, in Figure \ref{fig:nca-interval}. 

\begin{figure}[!htbp]
    \centering
    \includegraphics[width=\linewidth]{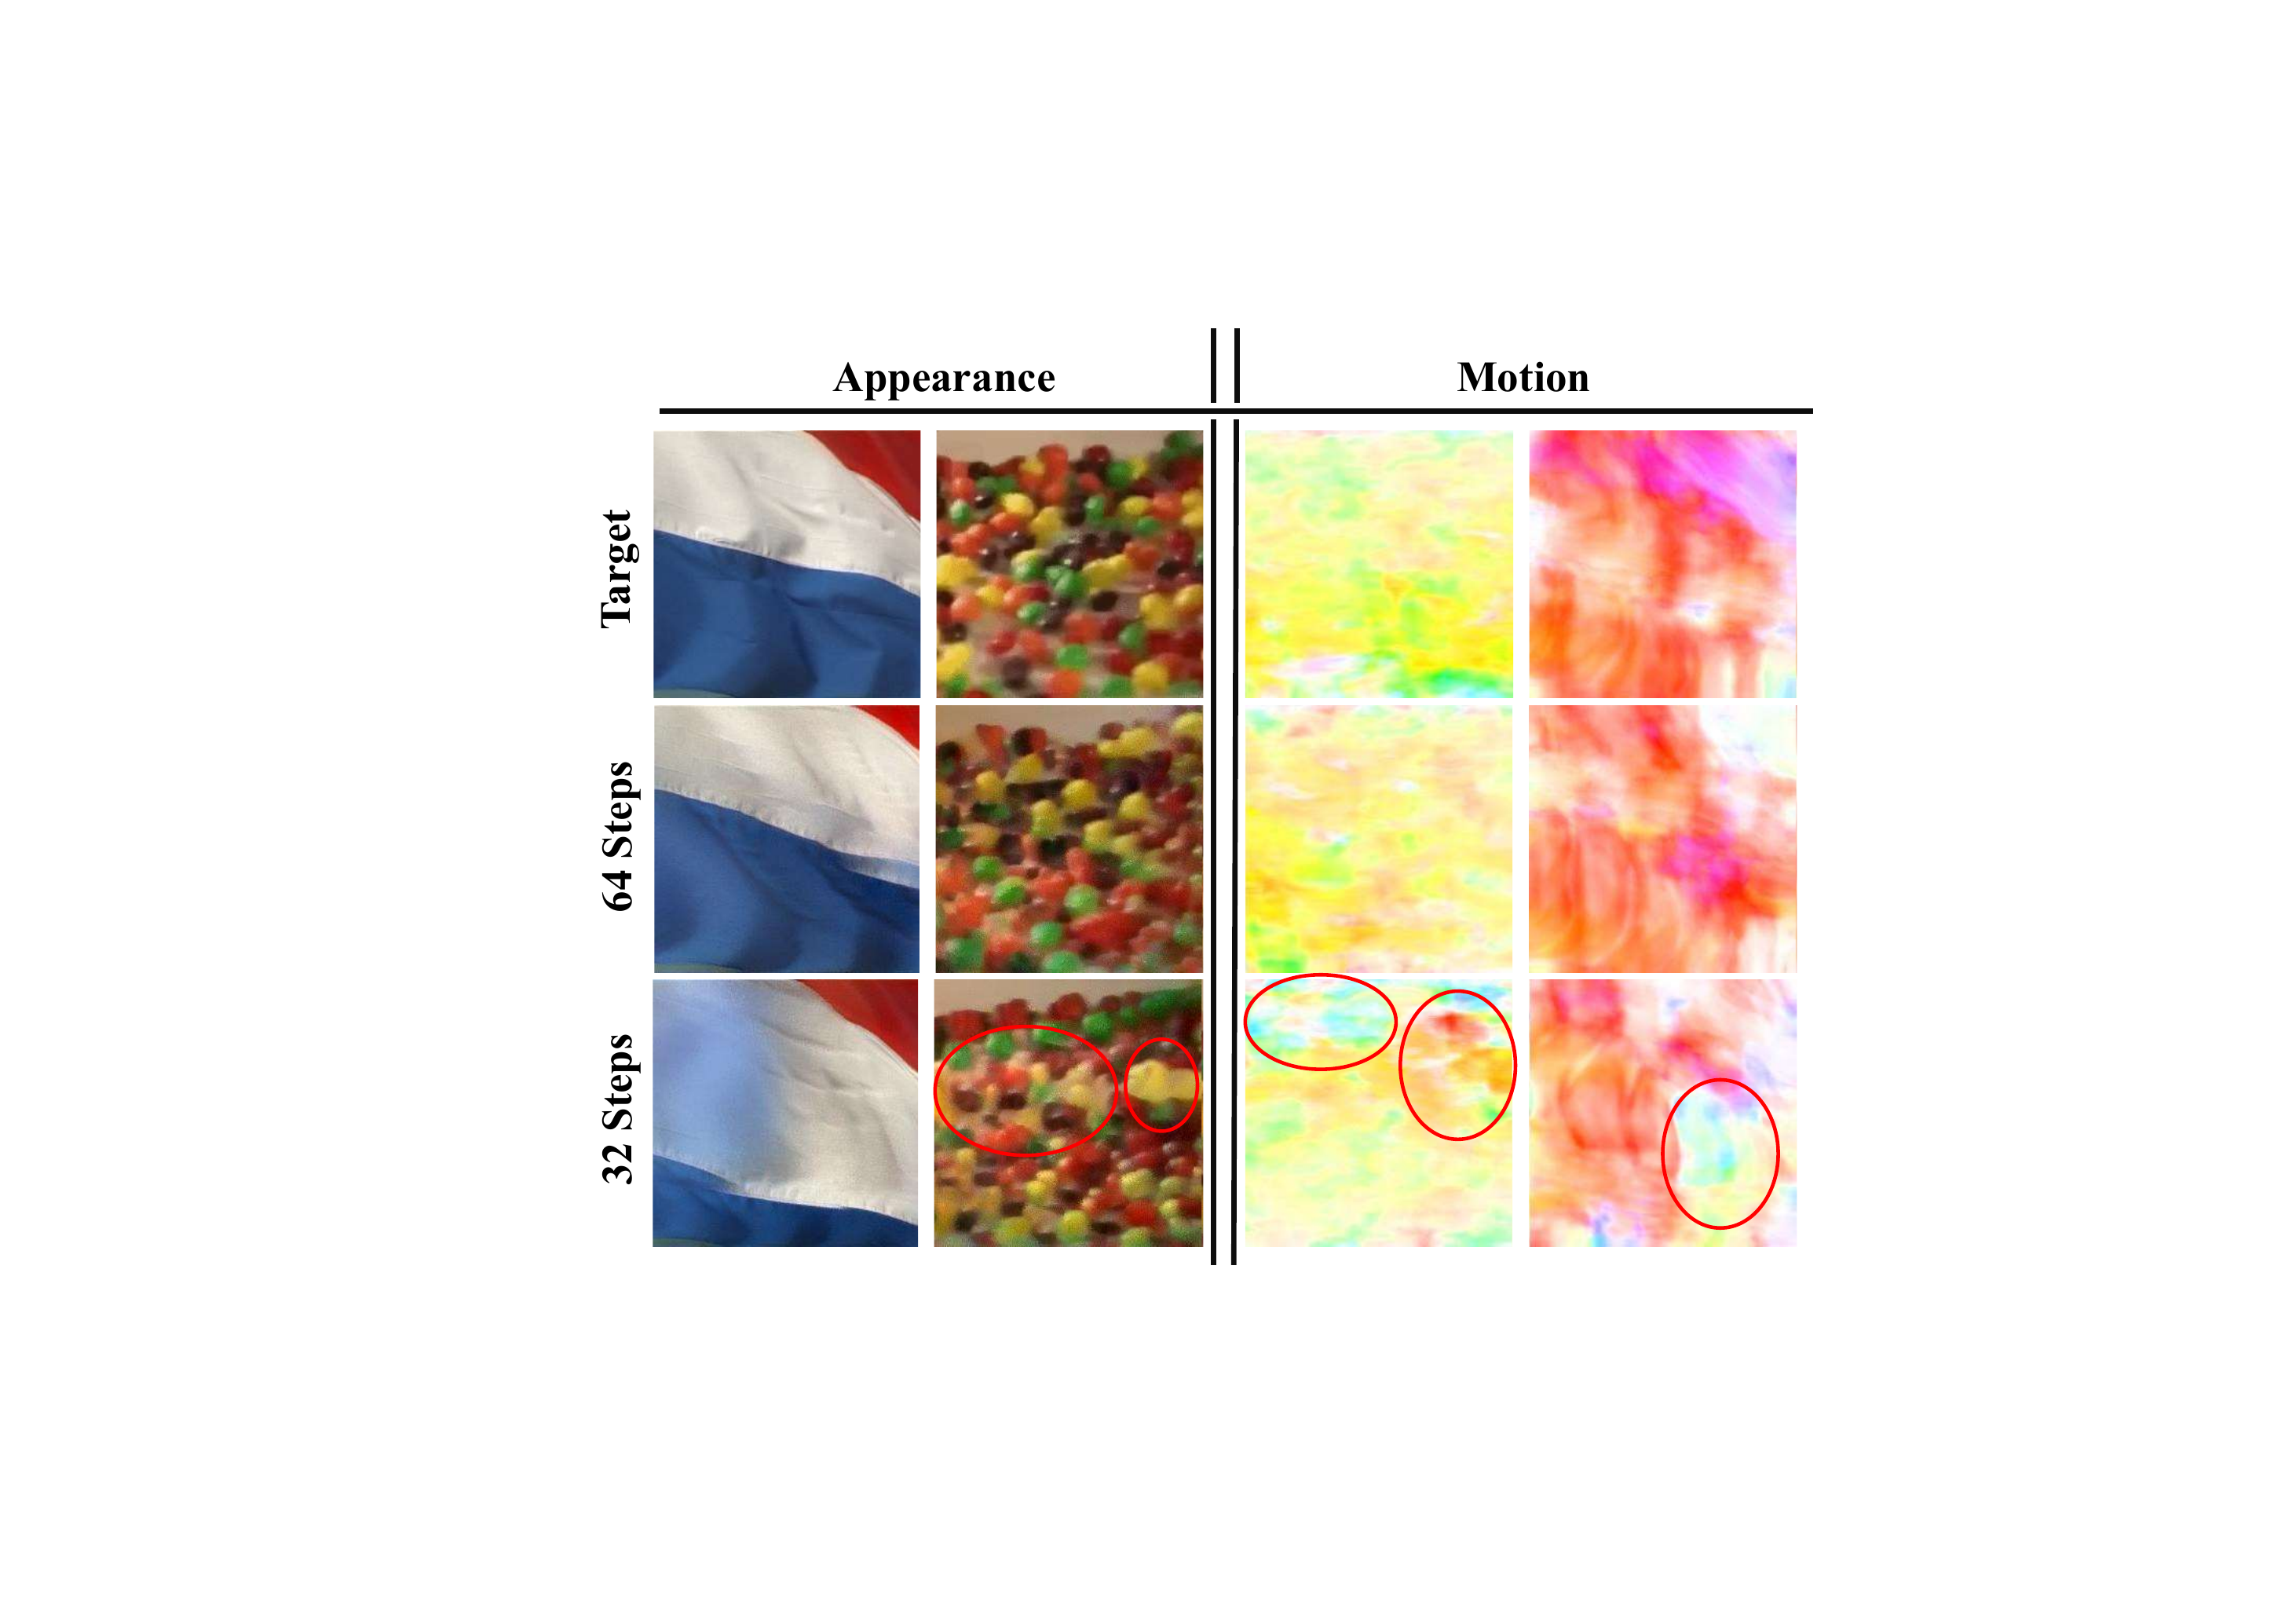}
    \caption{Comparison between training with 32 and 64 DyNCA time intervals for fitting one frame. Fewer DyNCA steps lowers the quality of the synthesized frame and leads to wrong motion. The two columns of flow images come from water\_3 and flag\_2 in the dataset of \cite{two_stream}}
    \label{fig:nca-interval}
\end{figure}

We can see that with fewer DyNCA steps, the quality of the texture synthesis decreases and artifacts occur. We also observe that DyNCA might generate wrong motions than the target video after training with a small number of intervals. Therefore, we select the maximum DyNCA steps in DyNCA-L-$256^2$ to train on a single Nvidia-A100 without exceeding memory, which is limited to 64. We use the same setting across all DyNCA configurations to ensure consistency.

\subsubsection{Dynamic Style Transfer}
We use the videos in the dataset introduced in \cite{two_stream} as the sources of target motions and use the images in figure \ref{fig:dst-images} as the sources of target appearances. We use the same training settings for dynamic style transfer as in dynamic texture synthesis (DyTS), except for the weight setting scheme. The target appearance and target motion in dynamic style transfer might be incompatible with each other. Hence, the automatic weight setting scheme in DyTS can generate incorrect weight values, leading to low-quality results. Therefore, we manually set the motion loss weight $\lambda$ in dynamic style transfer experiments. Concrete values are given in table \ref{tab:dst-weight}. 

% Please add the following required packages to your document preamble:
% \usepackage{multirow}
\begin{table}[]
\resizebox{\linewidth}{!}{
\begin{tabular}{ccc}
\toprule
Target Dynamics               & Target Appearance & Weight \\ \midrule
                             \midrule
\multirow{5}{*}{flames}      & cartoon\_fire\_1    & 2.0    \\  
                             & cartoon\_fire\_2    & 3.0    \\  
                             & cartoon\_fire\_4    & 2.0    \\  
                             & cartoon\_fire\_5    & 0.5    \\  
                             & cartoon\_fire\_6    & 2.0    \\ 
                             \midrule
\multirow{3}{*}{fireplace\_1} & cartoon\_fire\_2    & 5.0    \\  
                             & cartoon\_fire\_4    & 8.0    \\  
                             & cartoon\_fire\_6    & 8.0    \\ 
                             \midrule
\multirow{4}{*}{fireplace\_2} & cartoon\_fire\_2    & 10.0   \\  
                             & cartoon\_fire\_3    & 9.0    \\  
                             & cartoon\_fire\_4    & 5.0    \\  
                             & cartoon\_fire\_6    & 9.0    \\ 
                             \midrule
\multirow{4}{*}{sea\_2}       & cartoon\_water\_1   & 3.0    \\  
                             & cartoon\_water\_2   & 3.0    \\  
                             & cartoon\_water\_3   & 6.0    \\  
                             & cartoon\_water\_4   & 3.0    \\ 
                             \midrule
\multirow{3}{*}{water\_3}     & cartoon\_water\_1   & 3.0    \\  
                             & cartoon\_water\_3   & 0.5    \\  
                             & cartoon\_water\_4   & 0.5    \\
                             
\bottomrule
\end{tabular}
}
\caption{Weight settings of dynamic style transfer with DyNCA-L-256. All target dynamics come from the dataset introduced in \cite{two_stream}. Target appearance images refer to figure \ref{fig:dst-images}.}
\label{tab:dst-weight}
\end{table}

\begin{figure*}[!t]
    \centering
    \includegraphics[width=1.0\linewidth]{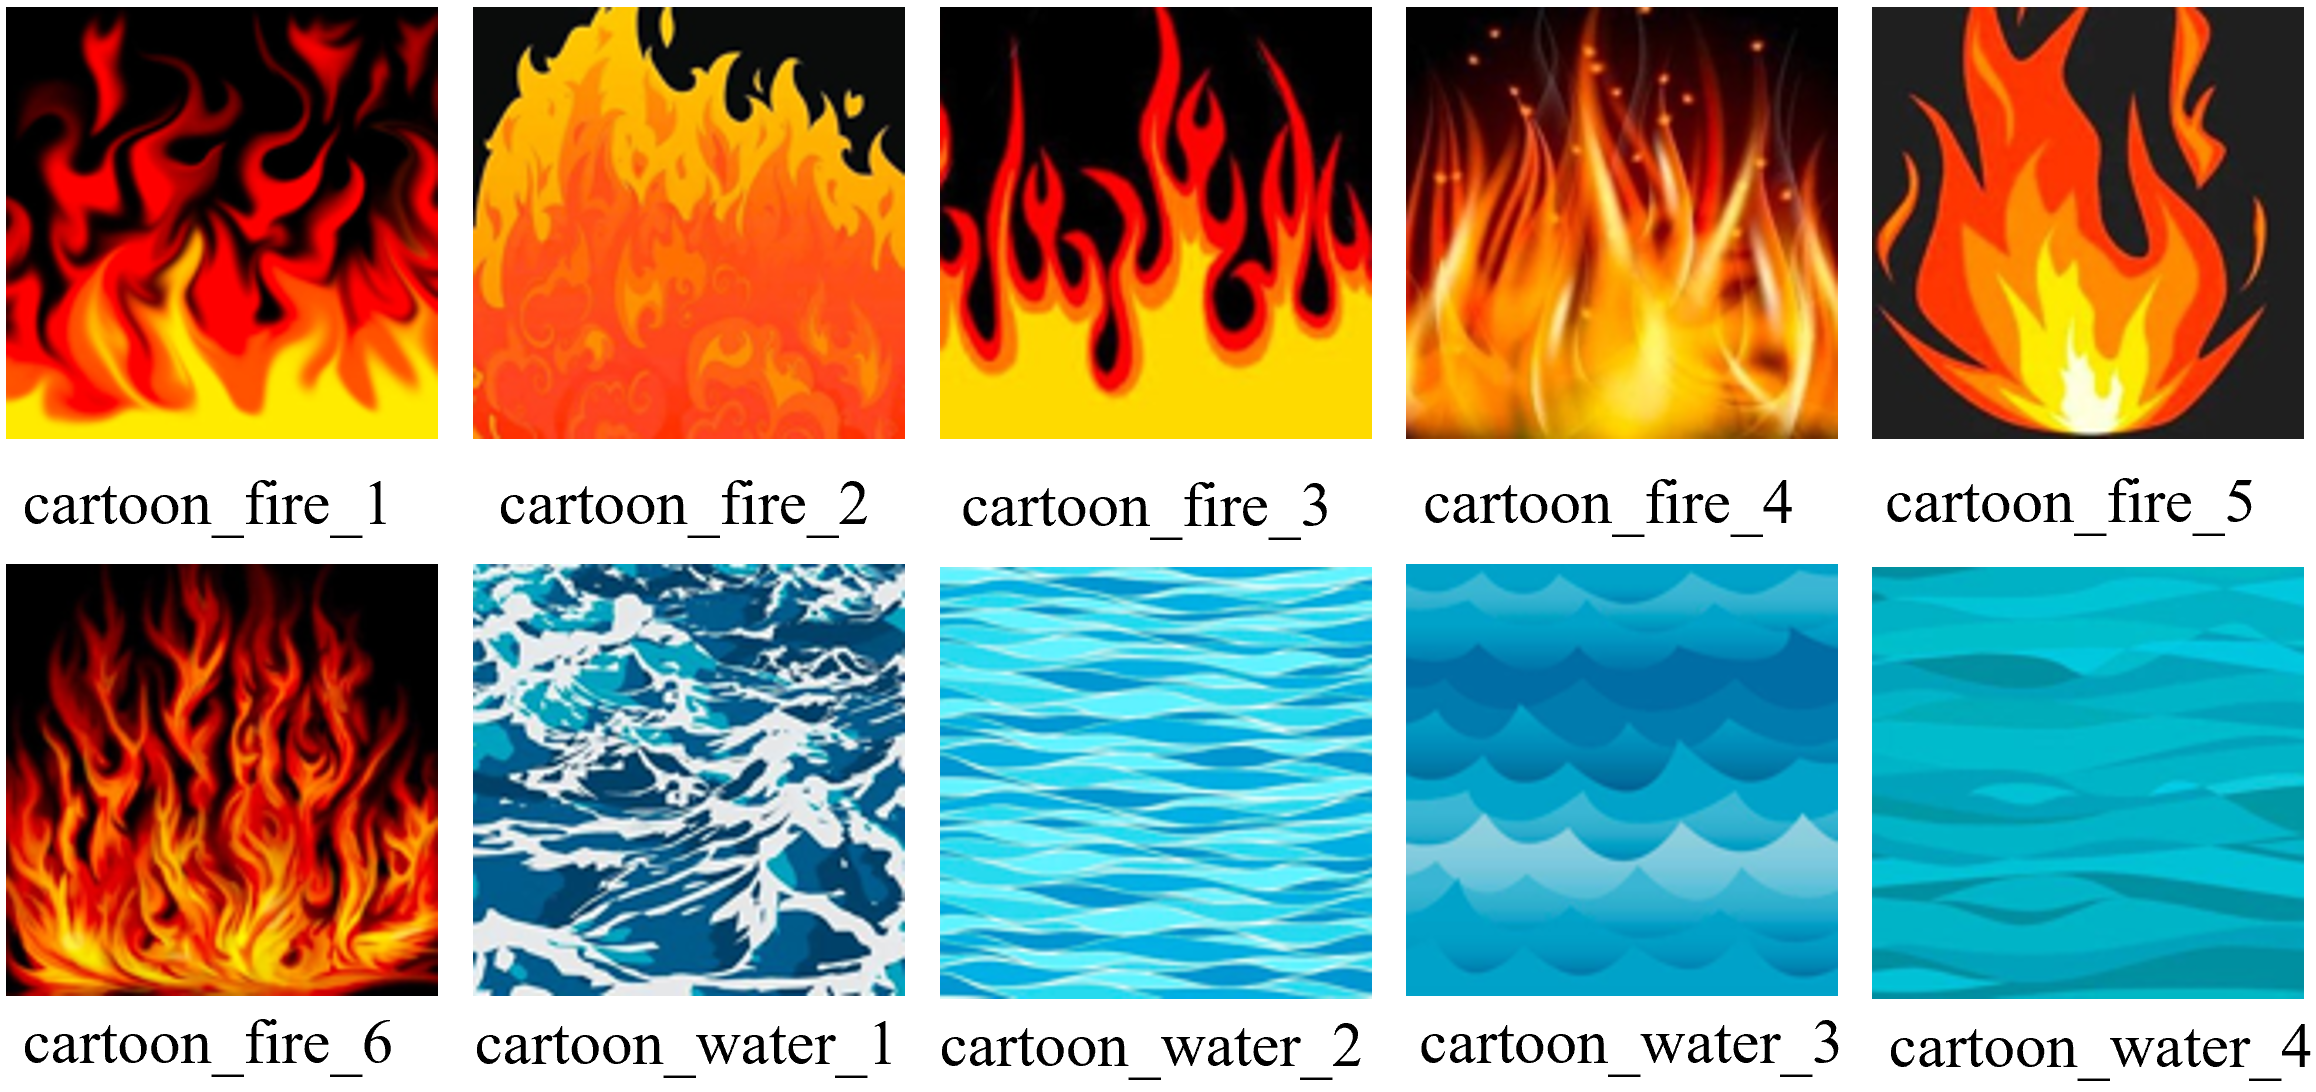}
    \caption{Target appearance images used in dynamic style transfer with DyNCA. Our dynamic style transfer synthesized videos are available at \href{https://dynca.github.io/\#style_transfer}{https://dynca.github.io/\#style\_transfer}.
    }
    \label{fig:dst-images}
\end{figure*}

\subsection{Limitations}
Although we have a scheme to automatically set the motion loss weight $\lambda$, we observe that the automatic weight leads to poor results in 7 of the 59 video textures in the dataset introduced in \cite{two_stream}. This can cause low-quality synthesized videos or diverging synthesis. Diverging synthesis means that DyNCA cannot generate meaningful patterns during video synthesis after a certain number of timesteps. 

To solve this problem, we manually set the motion loss weight $\lambda$ for those 7 videos on both DyNCA-S and DyNCA-L configurations. We show the concrete values of the manually set weights for each of these 7 dynamic texture videos in Table~\ref{tab:low-quality-weight}, and Table~\ref{tab:diverging-weight}. Table~\ref{tab:low-quality-weight} shows both the manual and automatically set weights for 2 of the 7 videos that yield low-quality results when we use the automatic weight setting scheme.
Table~\ref{tab:diverging-weight} shows both the manual and automatically set weights for 5 of the 7 videos that yield diverging results when we use the automatic weight setting scheme.

\begin{table}[]
\centering
\resizebox{\linewidth}{!}{
\begin{tabular}{cc||cc}
\toprule
\begin{tabular}[c]{@{}c@{}}NCA\\ Configs\end{tabular} & Weight Scheme & flames & sea\_2 \\ \midrule
                   \midrule
\multirow{2}{*}{S-256}                                & Automatic     & 5.5    & 2.1    \\ 
                                                      & Manual        & 3.0    & 4.0    \\ 
                   \midrule
\multirow{2}{*}{L-256}                                & Automatic     & 5.7    & 2.0    \\ 
                                                      & Manual        & 2.0    & 4.0    \\
\bottomrule                                                      
\end{tabular}
}
\caption{Two low-quality textures when using automatic weight settings. After manually tuning the weights, DyNCA can synthesize realistic video textures.}
\label{tab:low-quality-weight}
\end{table}

\begin{table*}[]
\centering
\resizebox{\textwidth}{!}{
\begin{tabular}{cc||ccccc}
% \hline
\toprule
\begin{tabular}[c]{@{}c@{}}NCA\\ Configs\end{tabular} & Weight Scheme & ants & sky\_clouds\_1 & smoke\_2 & smoke\_3 & calm\_water\_2 \\ \midrule
                    \midrule
\multirow{2}{*}{S}                                & Automatic     & 4.6  & 10.0           & 5.8      & 7.9      & 6.7            \\ 
                                                      & Manual        & 0.2  & 0.25           & 0.1      & 0.5      & 1.0            \\ 
                    \midrule
\multirow{2}{*}{L}                                & Automatic     & 4.1  & 10.0           & 6.8      & 6.5      & 6.6            \\ 
                                                      & Manual        & 0.2  & 0.25           & 0.1      & 1.0      & 1.0            \\ 
\bottomrule
\end{tabular}
}

\caption{Five textures that will diverge during video synthesis when using automatic weight settings. After manually tuning the weight, DyNCA can robustly synthesize realistic video textures.}
\label{tab:diverging-weight}
\end{table*}
