# Supplementary material for: DyNCA: Real-time Dynamic Texture Synthesis Using Neural Cellular Automata
Source: arXiv:2211.11417 source file (2023-03-30)
Supplement: Supplementary file 8 [file UserStudy.tex]

\section{User Study}
We follow the user-study settings introduced by Tesfaldet et al. \cite{two_stream}. The participants see two videos in random order, one after another, and are asked to choose the video that appears more realistic. Tesfaldet et al. \cite{two_stream} in their study use 12-frame videos with 10 frames-per-second (fps), resulting in videos of 1.2 seconds in length. However, they loop these videos to create longer videos in order to study the effect of exposure time. Their results show that for exposure times $\geq$ 1.2 seconds, the accuracy of the participants in detecting the real video saturates and does not improve much. Moreover, they only compare the videos synthesized by their method with the real videos.

Our user study is slightly different from the one conducted by Tesfaldet et al. \cite{two_stream}. \textbf{First}, we limit ourselves to the original video length (1.2 seconds) to avoid looping artifacts. This choice is also justified by the results from \cite{two_stream} since there is not much difference in their results for exposure times $\geq$ 1.2 seconds. 
\textbf{Second}, in addition to Tesfaldet et al. \cite{two_stream}, we experiment with videos synthesized by different SOTA methods to be able to compare their realism. We compare 4 different methods, including ours, with each other and with the real videos. These 4 methods are: DyNCA (Ours), (A) by Tesfaldet et al. \cite{two_stream}, (B) Config FC of STGConvNet by \cite{xie2017generativeconvnet}, (C) Config ST of STGConvNet by \cite{xie2017generativeconvnet}. Our choice of methods for comparison are based on two factors. First, Tesfaldet et al. \cite{two_stream} introduce the two-stream framework for dynamic texture synthesis and our framework incorporates its idea. Therefore, their method can be regarded as a baseline method in two-stream-based dynamic texture synthesis methods. Second, Xie et al.\cite{xie2017generativeconvnet} design a different framework than \cite{two_stream} via a generative-modeling perspective. While Zhang et al. \cite{zhang2021dynamic} have recently updated the two-stream-based method by using shifted Gram as the loss function and introducing a new frame sampling scheme, their model is fundamentally similar to of Tesfaldet et al. \cite{two_stream}. Hence, we have only considered the two main SOTA DyTS methods in the literature \cite{two_stream, xie2017generativeconvnet} for our comparisons.

% excluded it from our comparison as it would be redundant to include it alongside the method from \cite{two_stream}.

We conduct our user study on the Amazon Mechanical Turk (AMT) platform. We use the same 59 dynamic texture videos provided by Tesfaldet et al. \cite{two_stream}.
Each participant sees 59 pairs of videos. Similar to \cite{two_stream}, the first 3 videos are warm-up comparisons and are not considered in the final results. As suggested in \cite{two_stream}, we also chose 3 videos with very low quality, where the quality discrepancy is evident, as sentinel videos. We thus only consider the responses of participants who provide correct answers to those 3 sentinel videos. We then use the remaining 53 video comparisons in the evaluation. 

We randomly create 100 different experiments by shuffling the order of 59 videos and also by shuffling the video pairs for each of the 59 videos. Each of the experiments can be done by a maximum of 3 different participants, and we do not allow the participants to participate more than once in our user study. Given the constraints above on the AMT platform, we received valid responses from 163 unique participants,  which makes the total number of pairwise comparisons equal to $163 \times 53 = 8639$. 

Table~\ref{tab:user-study-supp} shows the results. Each entry in the table indicates the number of times that the video of the corresponding column is chosen over the video of the corresponding row as the more realistic video. The realism score presented in the last row shows the overall percentage that the corresponding column was chosen as the more realistic video. These results demonstrate that DyNCA has the highest realism score (54.9\%) among the DyTS methods.

\begin{figure}[htp]
\subfloat{%
\resizebox{\linewidth}{!}{
\begin{tabular}{cc||cccc}
\toprule
{} &  Real &  DyNCA &  A \cite{two_stream} &  B \cite{xie2017generativeconvnet} &  C \cite{xie2017generativeconvnet} \\
\midrule
Real                              &     N/A &    249 &                  218 &                                196 &                                 69 \\
DyNCA                             &   680 &      N/A &                  342 &                                394 &                                175 \\
A \cite{two_stream}               &   625 &    520 &                    N/A &                                413 &                                231 \\
B \cite{xie2017generativeconvnet} &   624 &    469 &                  381 &                                  N/A &                                127 \\
C \cite{xie2017generativeconvnet} &   819 &    695 &                  680 &                                732 &                                  N/A \\
\midrule
\textbf{Total Won} & 2748 & 1933 & 1621 & 1735 &  602 \\
\textbf{Total Lost} & 732 & 1591 & 1789 & 1601 & 2926 \\
\midrule
\textbf{Realism Score} & \begin{tabular}[c]{@{}c@{}} 79.0\%    \\ $\pm 0.7\%$\end{tabular}  & \begin{tabular}[c]{@{}c@{}} 54.9\%    \\ $\pm 0.8\%$\end{tabular} & \begin{tabular}[c]{@{}c@{}} 47.5\%    \\ $\pm 0.9\%$\end{tabular} & \begin{tabular}[c]{@{}c@{}} 52.0\%    \\ $\pm 0.9\%$\end{tabular} & \begin{tabular}[c]{@{}c@{}} 17.1\%    \\ $\pm 0.6\%$\end{tabular} \\
\bottomrule
\end{tabular}  
}}
\captionof{table}{Pair-wise comparison results from our user study. The participants see two videos, one after another, in random order and are asked to choose the video that appears more realistic. Each entry in the table shows the number of times that the video of the corresponding column was chosen over the video of the corresponding row as the more realistic video. The realism score presented in the last row shows the overall percentage that the corresponding column was chosen as the more realistic video. Our DyNCA achieves the highest realism score compared to the other DyTS methods (54.9\%).
}
\label{tab:user-study-supp}
\end{figure}
