# Supplementary material for: DyNCA: Real-time Dynamic Texture Synthesis Using Neural Cellular Automata
Source: arXiv:2211.11417 source file (2023-03-30)
Supplement: Supplementary file 10 [file Limitation.tex]

% \section{Limitations of DyNCA}
% Here we concretely give some results of failed cases of DyNCA.

% \textbf{Motion from vector field.}

% \textbf{Motion from video.} When learning motions from target videos, DyNCA is sensitive to the weight of motion loss, namely $\lambda$, when training with seed size of $256^2$. 
