# Supplementary material for: DyNCA: Real-time Dynamic Texture Synthesis Using Neural Cellular Automata
Source: arXiv:2211.11417 source file (2023-03-30)
Supplement: Supplementary file 11 [file MotionVidPosEmbAbl.tex]

\subsection{Motion from Video}
\label{suppsec:cpe-abl}

\subsubsection{Qualitative Analysis}
Without positional encoding, we observe several failed or distorted synthesized video frames, as shown in Figure \ref{fig:cpe-abl-vid}. Training without CPE can cause artifacts on synthesized frames and can lead to texture-less images of low quality.

\newcommand{\imgmvidcpevidabl}[1]{\includegraphics[height=70pt]{Supp/figures/MotionVidCPEAbl/#1}}

\newcolumntype{S}{>{\centering\arraybackslash} m{60pt} } 
\newcolumntype{Q}{>{\centering\arraybackslash} m{2pt} } 
\begin{table}[t]
\resizebox{\linewidth}{!}{
\begin{tabular}{m{2pt}SSSS}
    
% \toprule
    % \textbf{Target} &
    % \textbf{Single-scale} &
    % \textbf{Multi-scale} \\
    
    % \midrule
    
{\rotatebox{90}{\parbox{2.5cm}{\hspace{19pt} \textbf{Target}}}} &
\imgmvidcpevidabl{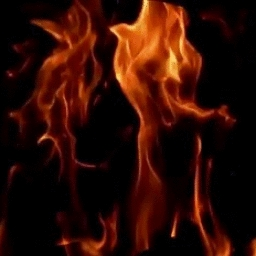}                                & \imgmvidcpevidabl{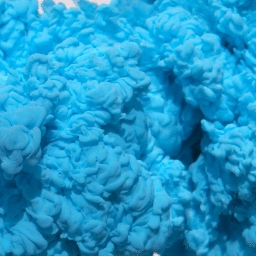}       & 
 \imgmvidcpevidabl{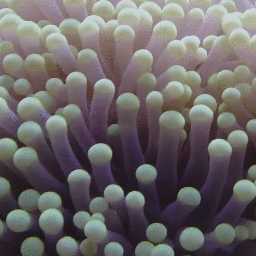}  &      
 \imgmvidcpevidabl{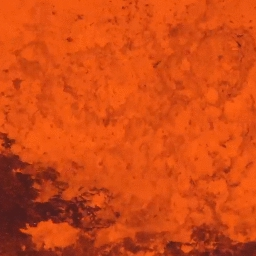} \\

% \midrule  

{\rotatebox{90}{\parbox{2.5cm}{\hspace{20pt} \textbf{Plain}}}} &
                          \imgmvidcpevidabl{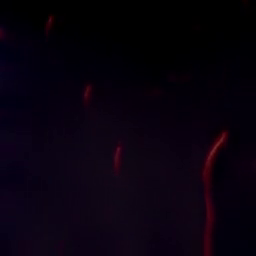}      & \imgmvidcpevidabl{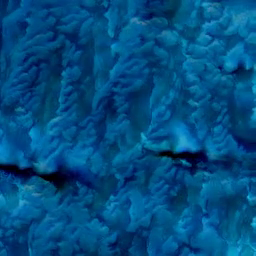}      &     \imgmvidcpevidabl{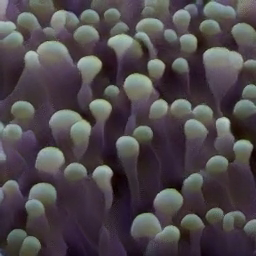}   &    \imgmvidcpevidabl{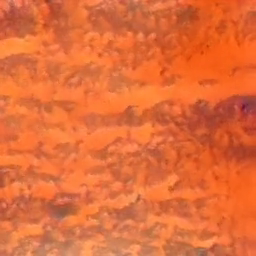}                \\
                            {\rotatebox{90}{\parbox{2.5cm}{\hspace{20pt} \textbf{CPE}}}} &
                           \imgmvidcpevidabl{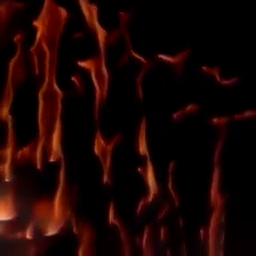} & \imgmvidcpevidabl{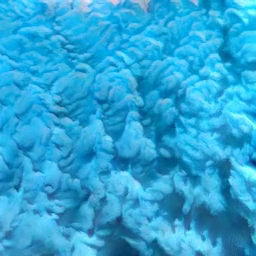}     & \imgmvidcpevidabl{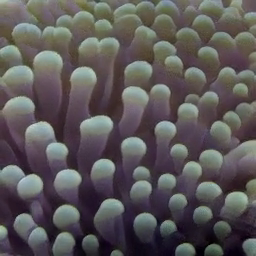}      &     \imgmvidcpevidabl{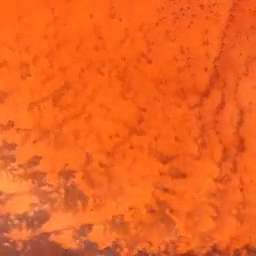}         
                            \\

\end{tabular}
}
\vspace{-10pt}
\captionof{figure}{Comparison between training with and without Cartesian Positional Encoding (CPE). The first row shows the target appearance texture. The results without CPE (second row) have less texture and more artifacts compared with the third row (with CPE). The results are obtained with DyNCA-S-256.}
\label{fig:cpe-abl-vid}
% \vspace{-10pt}
\end{table}

\subsubsection{Quantitative Analysis}

In Table~\ref{tab:pos-emb-abl-loss}, we record the loss values during video synthesis obtained from DyNCA trained with and without Cartesian Positional Encoding(CPE). The method for obtaining $\mathcal{L}_{appr}$ and $\mathcal{L}_{mvid}$ is the same as in the quantitative evaluation of the multi-scale perception ablation study, namely average across all ground-truth frames.

\begin{table}[htbp]
\begin{tabular}{c||cc||cc}
\toprule
\multirow{2}{*}{\begin{tabular}[c]{@{}c@{}}NCA \\ Configs\end{tabular}} & \multicolumn{2}{c||}{$\mathcal{L}_{appr}$}           & \multicolumn{2}{c}{$\mathcal{L}_{mvid}$}           \\ 
                                                                          & \multicolumn{1}{c}{CPE}  & Plain & \multicolumn{1}{c}{CPE}  & Plain \\ \midrule
                    \midrule
DyNCA-S-128                                                               & \multicolumn{1}{c}{\textbf{3.1762}} & {4.3809} & \multicolumn{1}{c}{\textbf{0.1670}} & 0.1874 \\ 
DyNCA-L-128                                                               & \multicolumn{1}{c}{\textbf{3.1789}} & 3.9818 & \multicolumn{1}{c}{\textbf{0.1654}} & 0.1834 \\ 
DyNCA-S-256                                                               & \multicolumn{1}{c}{\textbf{2.5536}} & 2.9358 & \multicolumn{1}{c}{\textbf{0.1959}} & 0.2102 \\ 
DyNCA-L-256                                                               & \multicolumn{1}{c}{\textbf{2.5633}} & 2.8756 & \multicolumn{1}{c}{\textbf{0.1901}} & 0.1980 \\ 
\bottomrule
\end{tabular}
\caption{Loss values during video synthesis after training. "Plain" refers to not adding positional encoding to cell states. CPE contributes to a better fitting of target appearance and motion.}
\label{tab:pos-emb-abl-loss}
\end{table}

In all DyNCA settings, positional encoding helps decrease the test loss during video synthesis, indicating the importance of our proposed positional encoding method.
